# Supplementary material for: FedORGP: Guiding Heterogeneous Federated Learning with Orthogonality Regularization on Global Prototypes
Source: arXiv:2502.16119 source file (2025-04-01)
Supplement: Supplementary file 1 [file X_suppl.tex]

\setcounter{page}{1}
\maketitlesupplementary

\section{More Experimental Results}
\label{sec:more experimental results}
\subsection{Impact of Local Epochs}
We evaluated the accuracy variation across all algorithms under different numbers of local training sessions. Notably, only a single global training iteration was conducted to mitigate the significant computational cost associated with frequent local updates. Experimental results reveal that when $E=5$, the accuracy of all baselines improved, whereas FedOC experienced a decline. This may be attributed to the insufficient training of orthogonal constraints, leading to inadequate prototype separation and excessive client alignment with prototypes, ultimately causing feature space overlap. As $E$ increases to 10, the accuracy variation across all algorithms becomes more stable.

\begin{table}[ht]
\caption{The test accuracy (\%) on Cifar100 with various local epochs under the pathological setting.}
\label{tab:test various local epochs} % 设置标签以便引用
\centering
\resizebox{0.4\linewidth}{!}{%
\begin{tabular}{|l|lll|}
\hline
          & \multicolumn{3}{c|}{Various Local Epochs}                                             \\ \hline
Settings  & \multicolumn{1}{c|}{$E = 1$}          & \multicolumn{1}{c|}{$E = 5$}          & \multicolumn{1}{c|}{$E = 10$}         \\ \hline
FML       & \multicolumn{1}{l|}{49.49} & \multicolumn{1}{l|}{53.76} & 53.59 \\ \hline
LG-FedAvg & \multicolumn{1}{l|}{54.81} & \multicolumn{1}{l|}{55.29} & 55.29 \\ \hline
FedGen    & \multicolumn{1}{l|}{54.99} & \multicolumn{1}{l|}{55.52} & 55.40 \\ \hline
FedProto  & \multicolumn{1}{l|}{52.63} & \multicolumn{1}{l|}{52.66} & 52.42 \\ \hline
FedKD     & \multicolumn{1}{l|}{50.28} & \multicolumn{1}{l|}{55.07} & 55.58 \\ \hline
FedGH     & \multicolumn{1}{l|}{54.87} & \multicolumn{1}{l|}{55.27} & 55.56 \\ \hline
FedTGP    & \multicolumn{1}{l|}{51.18} & \multicolumn{1}{l|}{54.54} & 53.72 \\ \hline
FedOC   & \multicolumn{1}{l|}{\textbf{62.34}}   & \multicolumn{1}{l|}{\textbf{58.07}}   & \textbf{58.17}   \\ \hline
\end{tabular}
}
\end{table}

\subsection{Impact of Orthogonality Constraints Rounds}
We trained FedOC across three datasets with varying rounds of orthogonal constraints to explore their impact on client model training. The highest model accuracy is observed when $SE=1$. However, as $SE$ increases, model accuracy declines. Excessive angular separation between inter-class prototypes leads to a loss of adaptability to the local data distribution on the client side, hindering the ability to capture the specific characteristics of local data and reducing the global model's generalizability.

\begin{table}[ht]
\caption{The test accuracy (\%) of FedOC across three datasets in the pathological setting is used to evaluate the impact of server epochs on client model performance.}
\label{tab:test various server epochs} % 设置标签以便引用
\centering
\resizebox{0.55\linewidth}{!}{%
\begin{tabular}{|l|lll|}
\hline
          & \multicolumn{3}{c|}{Various Server Epochs ($SE$)}                                             \\ \hline
Settings  & \multicolumn{1}{c|}{$SE = 1$}          & \multicolumn{1}{c|}{$SE = 10$}          & \multicolumn{1}{c|}{$SE = 100$}         \\ \hline
Cifar10       & \multicolumn{1}{l|}{\textbf{85.71 ± 0.10}} & \multicolumn{1}{l|}{85.00 ± 0.24} & 85.38 ± 0.17 \\ \hline
Cifar100 & \multicolumn{1}{l|}{\textbf{61.12 ± 0.15}} & \multicolumn{1}{l|}{60.44 ± 0.30} & 52.56 ± 0.36 \\ \hline
Flowers102    & \multicolumn{1}{l|}{\textbf{64.15 ± 1.66}} & \multicolumn{1}{l|}{63.92 ± 0.91} & 56.16 ± 1.19\\ \hline
\end{tabular}
}
\end{table}

\section{Convergence Analysis for FedOC}
\label{sec:convergence analysis}

\subsection{Proof for Lemma 1}
Since FedORGP makes no change to the local model training process, Lemma 1 derived by FedProto still holds.

\subsection{Proof for Lemma 2}
In this section, we demonstrate the impact of updating the global prototype under orthogonal constraints on client model training.

\begin{align}
&\mathcal{L}^{(t+1)E+0} - \mathcal{L}^{(t+1)E} \\
&= \lambda_c(1 - \langle r^{(t+1)E}, \mathcal{P}^{t+1}\rangle) - \lambda_c(1 - \langle r^{(t+1)E}, \mathcal{P}^{t}\rangle)\\
&= \lambda_c(\langle r^{(t+1)E}, \mathcal{P}^{t}\rangle - \langle r^{(t+1)E}, \mathcal{P}^{t+1}\rangle)\\
&\stackrel{(a)}{=} \lambda_c[(r^{(t+1)E})^T \cdot \mathcal{P}^t - (r^{(t+1)E})^T \cdot \mathcal{P}^{t+1}]\\
&= \lambda_c (r^{(t+1)E})^T (\mathcal{P}^t - \mathcal{P}^{t+1})\\
&= \lambda_c (r^{(t+1)E})^T \eta \nabla\mathcal{L}^{server}\\
&= \lambda_c \eta \|r^{t+1}\|\|\nabla\mathcal{L}^{server}\|cos\theta\\
&\stackrel{(b)}{\le} \lambda_c \eta G
\end{align}
(a):$r$ and $\mathcal{P}$ have been normalized.\\
(b):Since $r$ has been normalized, $\|r\|$ is 1. According to assumption 3(Bounded Expectation of Euclidean norm of Stochastic Gradients of the Global Prototype), $\|\nabla\mathcal{L}^{server}\| \le$ G. $\theta$ is the angle between the global prototype $\mathcal{P}$ and $r$, so $cos\theta \le$ 1.

Then we can get Eq. \ref{Eq:lemma 2 w/o Expection}

\begin{align}
    \mathcal{L}^{(t+1)E+0} \le \mathcal{L}^{(t+1)E} + \lambda_c \eta G
    \label{Eq:lemma 2 w/o Expection}
\end{align}

Take the expection of $B$ on both sides of Eq. \ref{Eq:lemma 2 w/o Expection}, we have

\begin{align}
    \mathbb{E}[\mathcal{L}^{(t+1)E+0}] \le \mathbb{E}[\mathcal{L}^{(t+1)E}] + \lambda_c \eta G
\end{align}

\subsection{Proof for Theorem 1}
Leveraging Lemma 1 and Lemma 2, we derive Theorem 1, which establishes an upper bound on the expected reduction in loss achieved during a single round of local training:

\begin{align}
    &\mathbb{E}\left[\mathcal{L}^{(t+1)E+0}\right] \\
    & \le \mathcal{L}^{tE+0} - \left(\eta - \frac{L_1 \eta^2}{2}\right) \sum_{e=0}^{E-1} \|\mathcal{L}^{tE+e}\|_2^2 + \frac{L_1 E \eta^2}{2} \sigma^2 + \lambda_c \eta G
\end{align}

\subsection{Proof for Theorem 2}
Theorem 1 can be re-expressed as:
\begin{align}
     &\left(\eta - \frac{L_1 \eta^2}{2}\right) \sum_{e=0}^{E-1} \|\mathcal{L}^{tE+e}\|_2^2 \\ 
     &\le \mathcal{L}^{tE+0} - \mathbb{E}\left[\mathcal{L}^{(t+1)E+0}\right] + \frac{L_1 E \eta^2}{2} \sigma^2 + \lambda_c \eta G
\end{align}

\begin{align}
     &\sum_{e=0}^{E-1} \|\mathcal{L}^{tE+e}\|_2^2 \\ 
      &\le \frac{\mathcal{L}^{tE+0} - \mathbb{E}\left[\mathcal{L}^{(t+1)E+0}\right] + \frac{L_1 E \eta^2}{2} \sigma^2 + \lambda_c \eta G}{\left(\eta - \frac{L_1 \eta^2}{2}\right)}
    \label{Eq:Theorem 2 before E}
\end{align}

Take expectations of model $\omega$ on both sides of Eq. \ref{Eq:Theorem 2 before E}, we have:

\begin{align}
     &\sum_{e=0}^{E-1} \mathbb{E}\|\mathcal{L}^{tE+e}\|_2^2 \\  & \le\frac{\mathbb{E}[\mathcal{L}^{tE+0}] - \mathbb{E}\left[\mathcal{L}^{(t+1)E+0}\right] + \frac{L_1 E \eta^2}{2} \sigma^2 + \lambda_c \eta G}{\left(\eta - \frac{L_1 \eta^2}{2}\right)}
    \label{Eq:Theorem 2 with E}
\end{align}
Summing both sides of Eq. \ref{Eq:Theorem 2 with E} over $T$ rounds ($t \in [0, T - 1]$), we have:
\begin{align}
     &\frac{1}{T}\sum_{t=0}^{T-1} \sum_{e=0}^{E-1} \mathbb{E}\|\mathcal{L}^{tE+e}\|_2^2 \\
     & \le \frac{\frac{1}{T}\sum_{t=0}^{T-1}(\mathbb{E}[\mathcal{L}^{tE+0}] - \mathbb{E}\left[\mathcal{L}^{(t+1)E+0}\right]) + \frac{L_1 E \eta^2}{2} \sigma^2 + \lambda_c \eta G}{\left(\eta - \frac{L_1 \eta^2}{2}\right)} \\
    & \stackrel{(c)}{\le} \frac{\frac{1}{T}(L^{t = 0} - L^*) + \frac{L_1 E \eta^2}{2} \sigma^2 + \lambda_c \eta G}{\left(\eta - \frac{L_1 \eta^2}{2}\right)} 
\end{align}

(c): Since $\sum_{t=0}^{T-1}(\mathbb{E}[\mathcal{L}^{tE+0}] - \mathbb{E}\left[\mathcal{L}^{(t+1)E+0}\right]) \le L^{t = 0} - L^*$

If the local model can converge, the above equation satisfies Eq. \ref{Eq:If local model convergence}

\begin{align}
    \frac{\frac{1}{T}(L^{t = 0} - L^*) + \frac{L_1 E \eta^2}{2} \sigma^2 + \lambda_c \eta G}{\left(\eta - \frac{L_1 \eta^2}{2}\right)} \le \epsilon
    \label{Eq:If local model convergence}
\end{align}

\begin{align}
    \frac{1}{T}(L^{t = 0} - L^*) \le & \epsilon\left(\eta - \frac{L_1 \eta^2}{2}\right) - \frac{L_1 E \eta^2}{2} \sigma^2 - \lambda_c \eta G
\end{align}

\begin{align}
    T \ge \frac{L^{t = 0} - L^*}{\epsilon\left(\eta - \frac{L_1 \eta^2}{2}\right) - \frac{L_1 E \eta^2}{2} \sigma^2 - \lambda_c \eta G}
\end{align}

Since $T > 0, L^{t = 0} - L^* > 0$, we can further derive that
\begin{align}
    \epsilon\left(\eta - \frac{L_1 \eta^2}{2}\right) - \frac{L_1 E \eta^2}{2} \sigma^2 - \lambda_c \eta G > 0
\end{align}

\begin{align}
    \eta < \frac{2(\epsilon - \lambda_c G)}{L1(\epsilon + E \sigma^2)}
\end{align}

\begin{align}
    \lambda_c < \frac{\epsilon}{G}
\end{align}

It shows that, when $\eta < \frac{2(\epsilon - \lambda_c G)}{L1(\epsilon + E \sigma^2)}$, $\lambda_c < \frac{\epsilon}{G}$, for an arbitrary client, the model can converge to a solution with a rate that is proportional to $O(1/T )$, where $T$ is the number of communication rounds.

\section{Visualization}
\label{sec:visualization}
We present the data distributions, encompassing both training and test datasets, as part of the experimental setup.

\begin{figure}[ht]
    \centering
    \includegraphics[width=\linewidth, height=10cm]{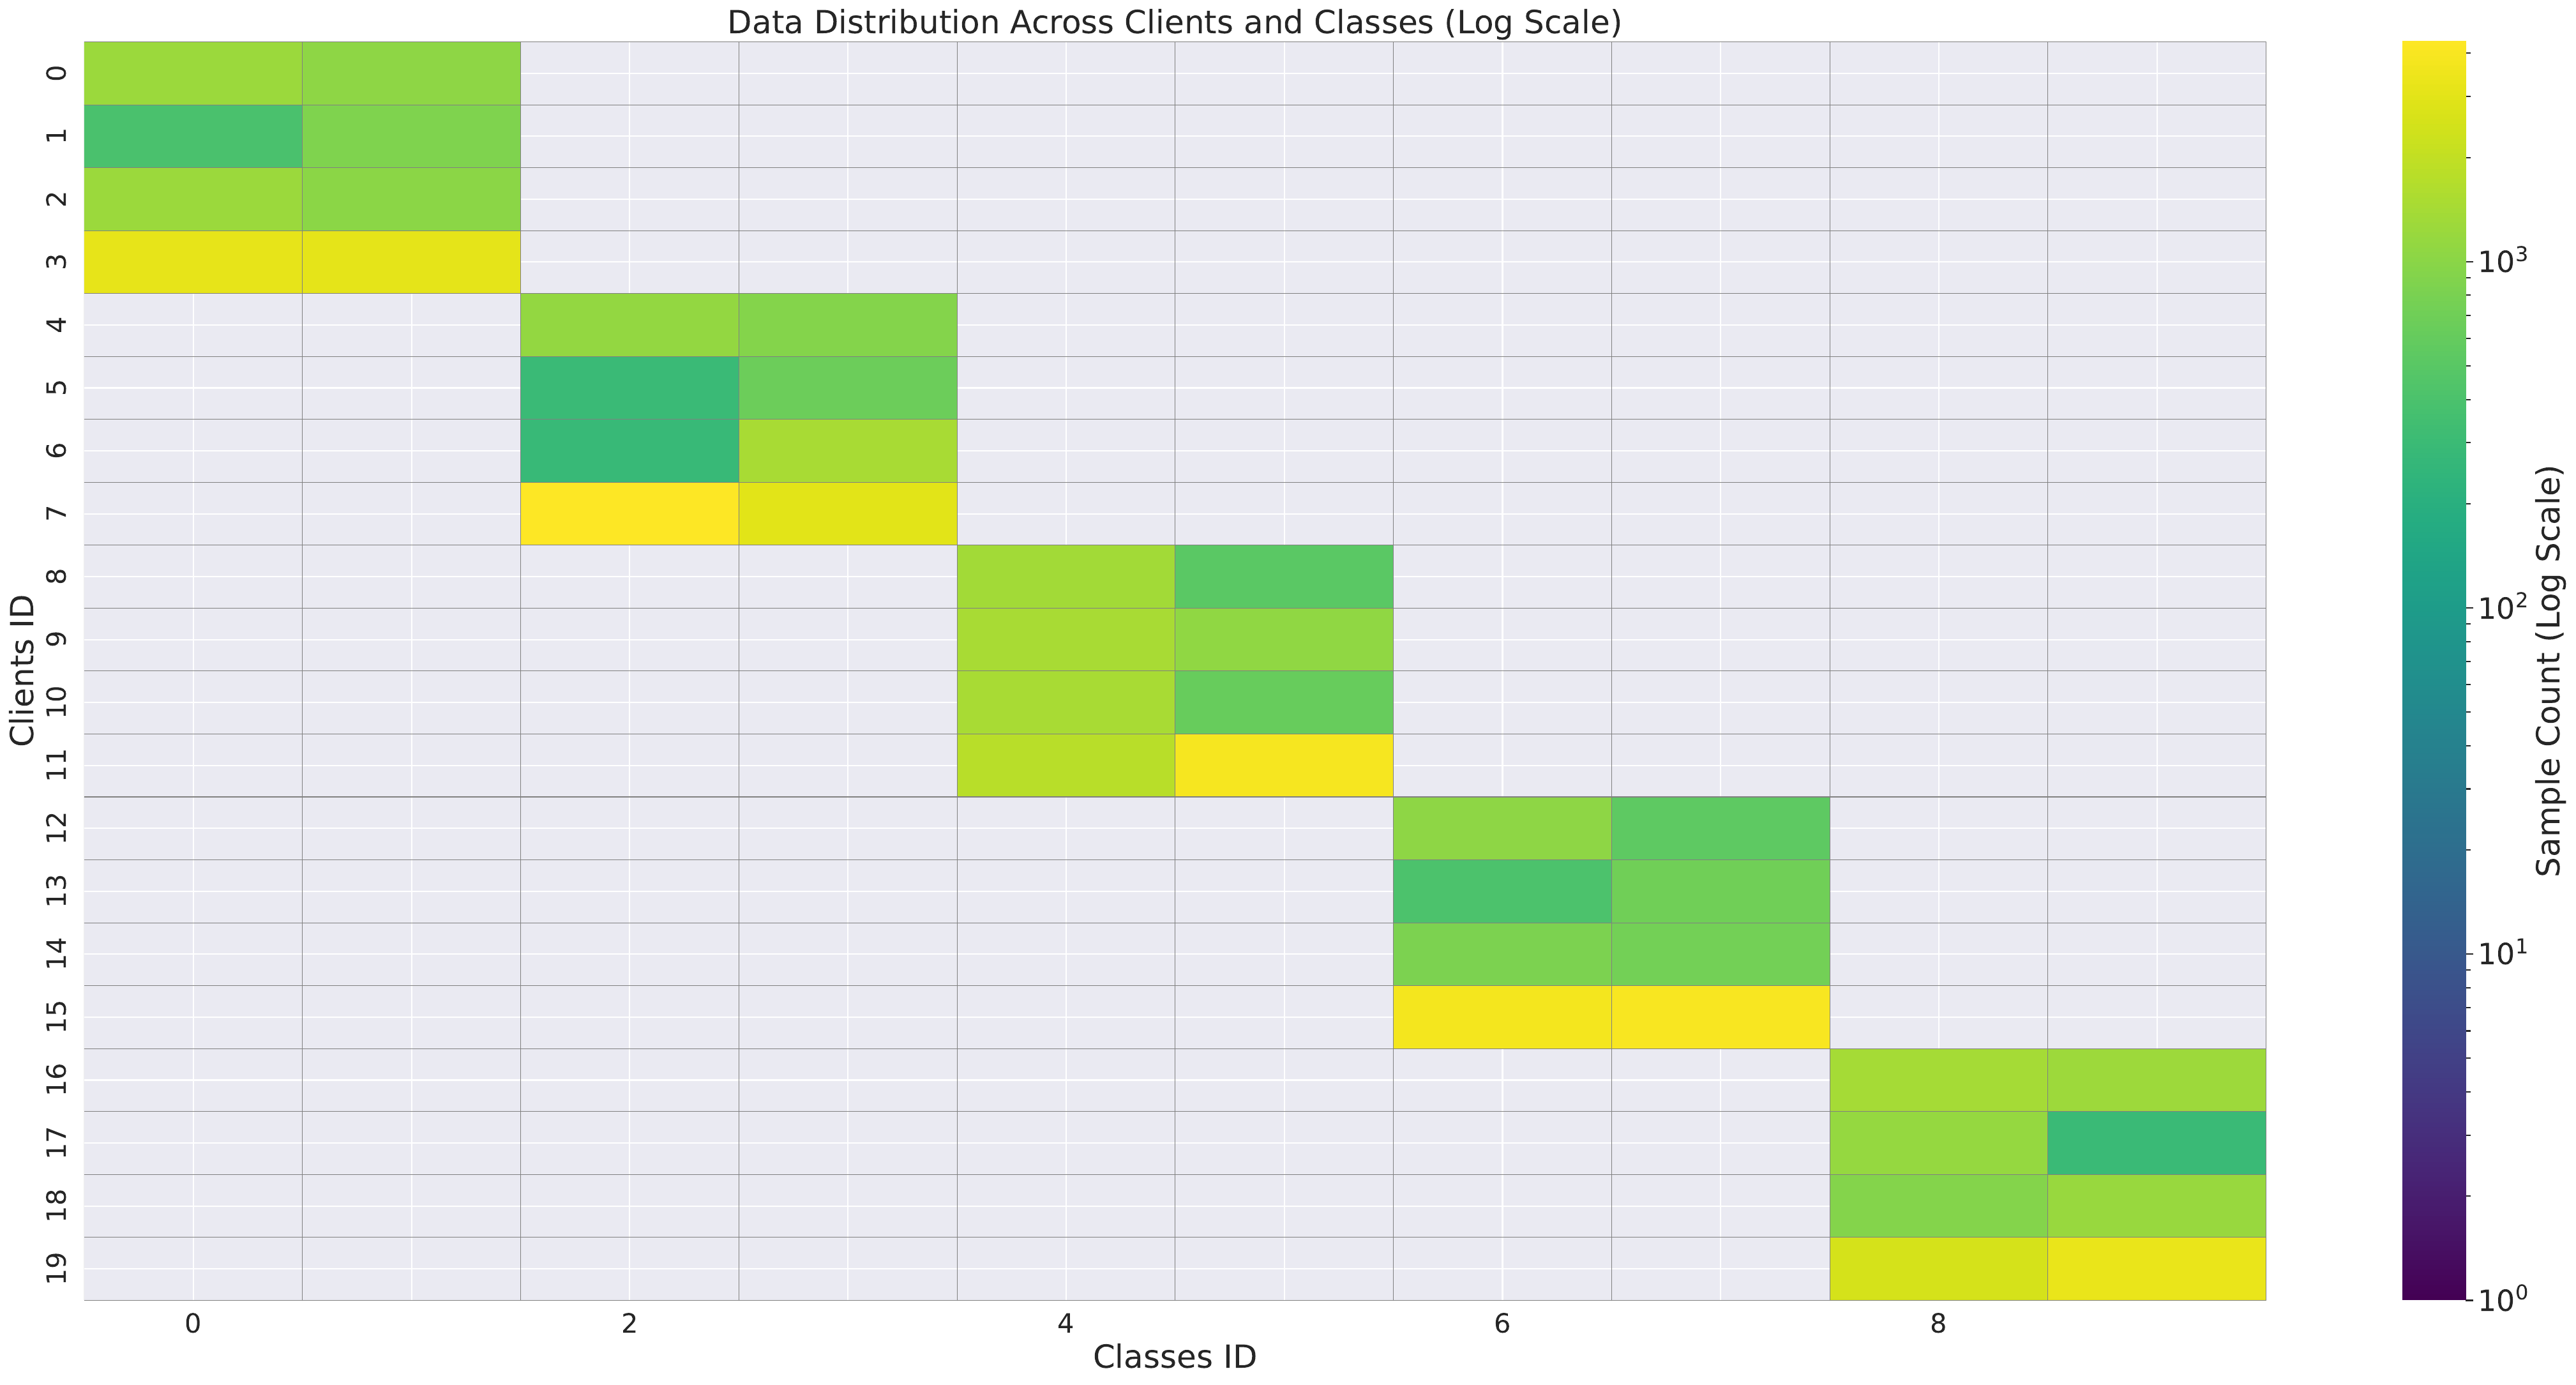}
    \caption{The data distribution for each client on the Cifar10 dataset is visualized under the pathological setting, where each client is assigned 2 classes. Brighter colors indicate larger sample sizes.}
    \label{fig:Cifar10_visualization}
\end{figure}

\begin{figure}[ht]
    \centering
    \includegraphics[width=\linewidth, height=10cm]{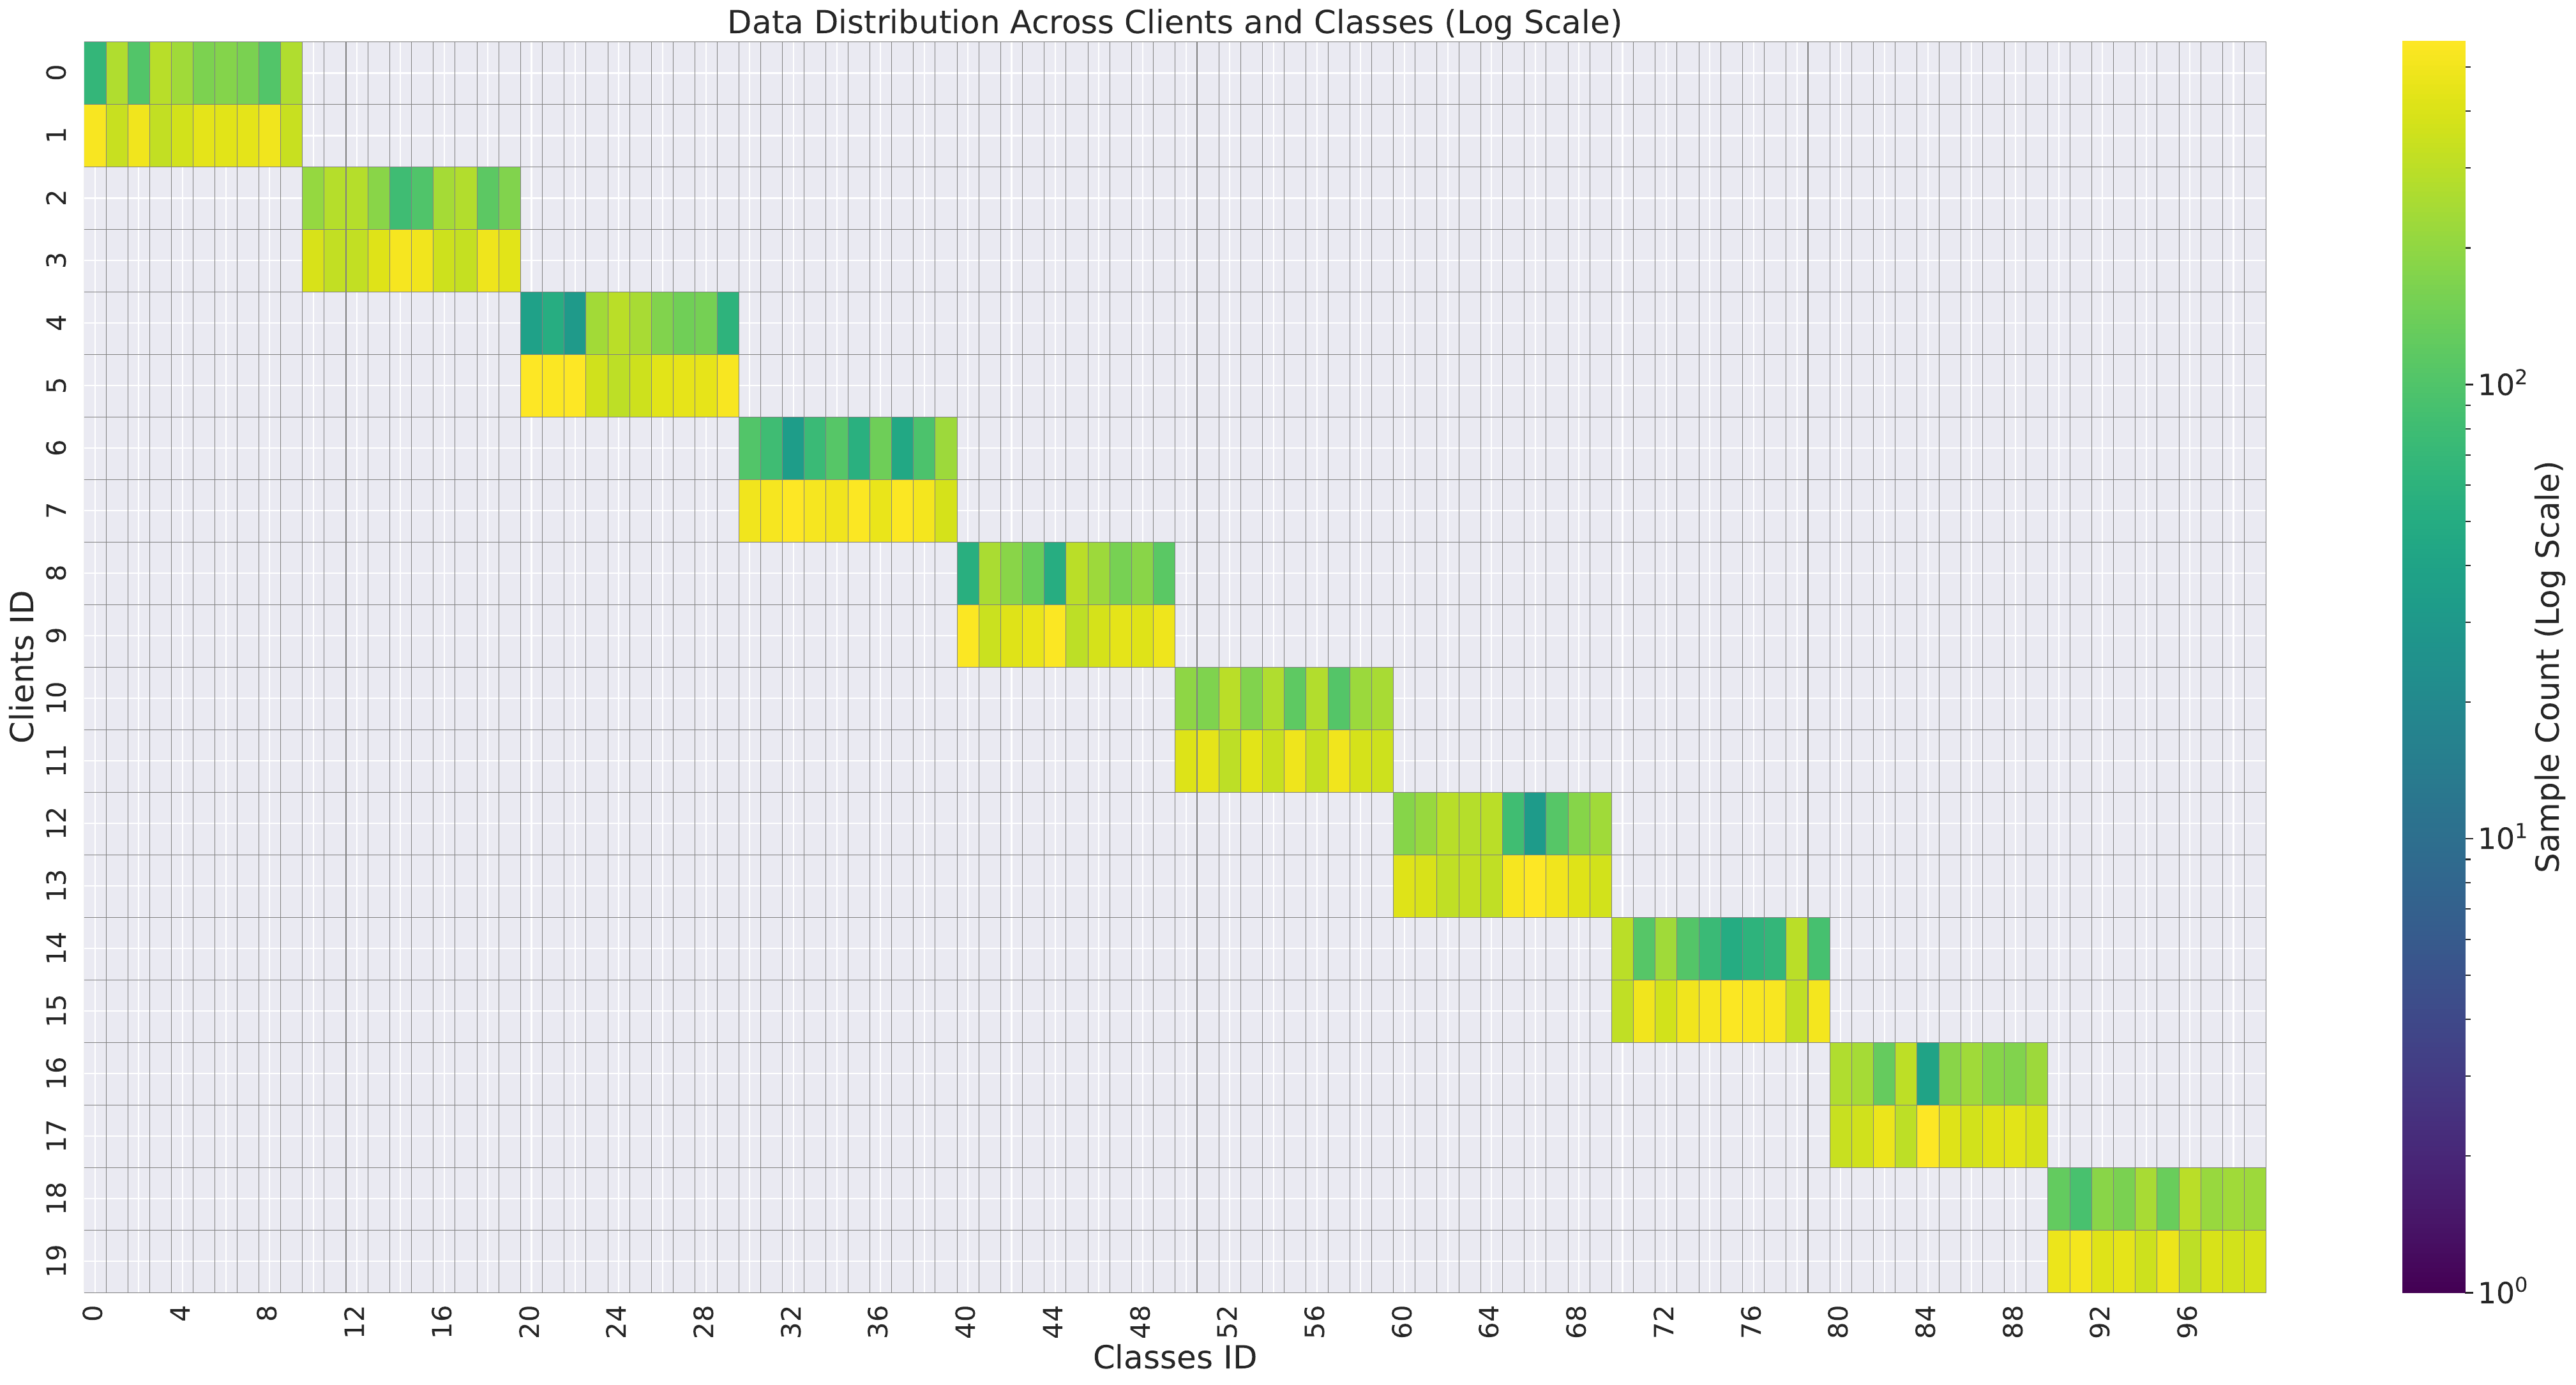}
    \caption{The data distribution for each client on the Cifar100 dataset is visualized under the pathological setting, where each client is assigned 10 classes. Brighter colors indicate larger sample sizes.}
    \label{fig:Cifar100_visualization}
\end{figure}

\begin{figure}[ht]
    \centering
    \includegraphics[width=\linewidth, height=10cm]{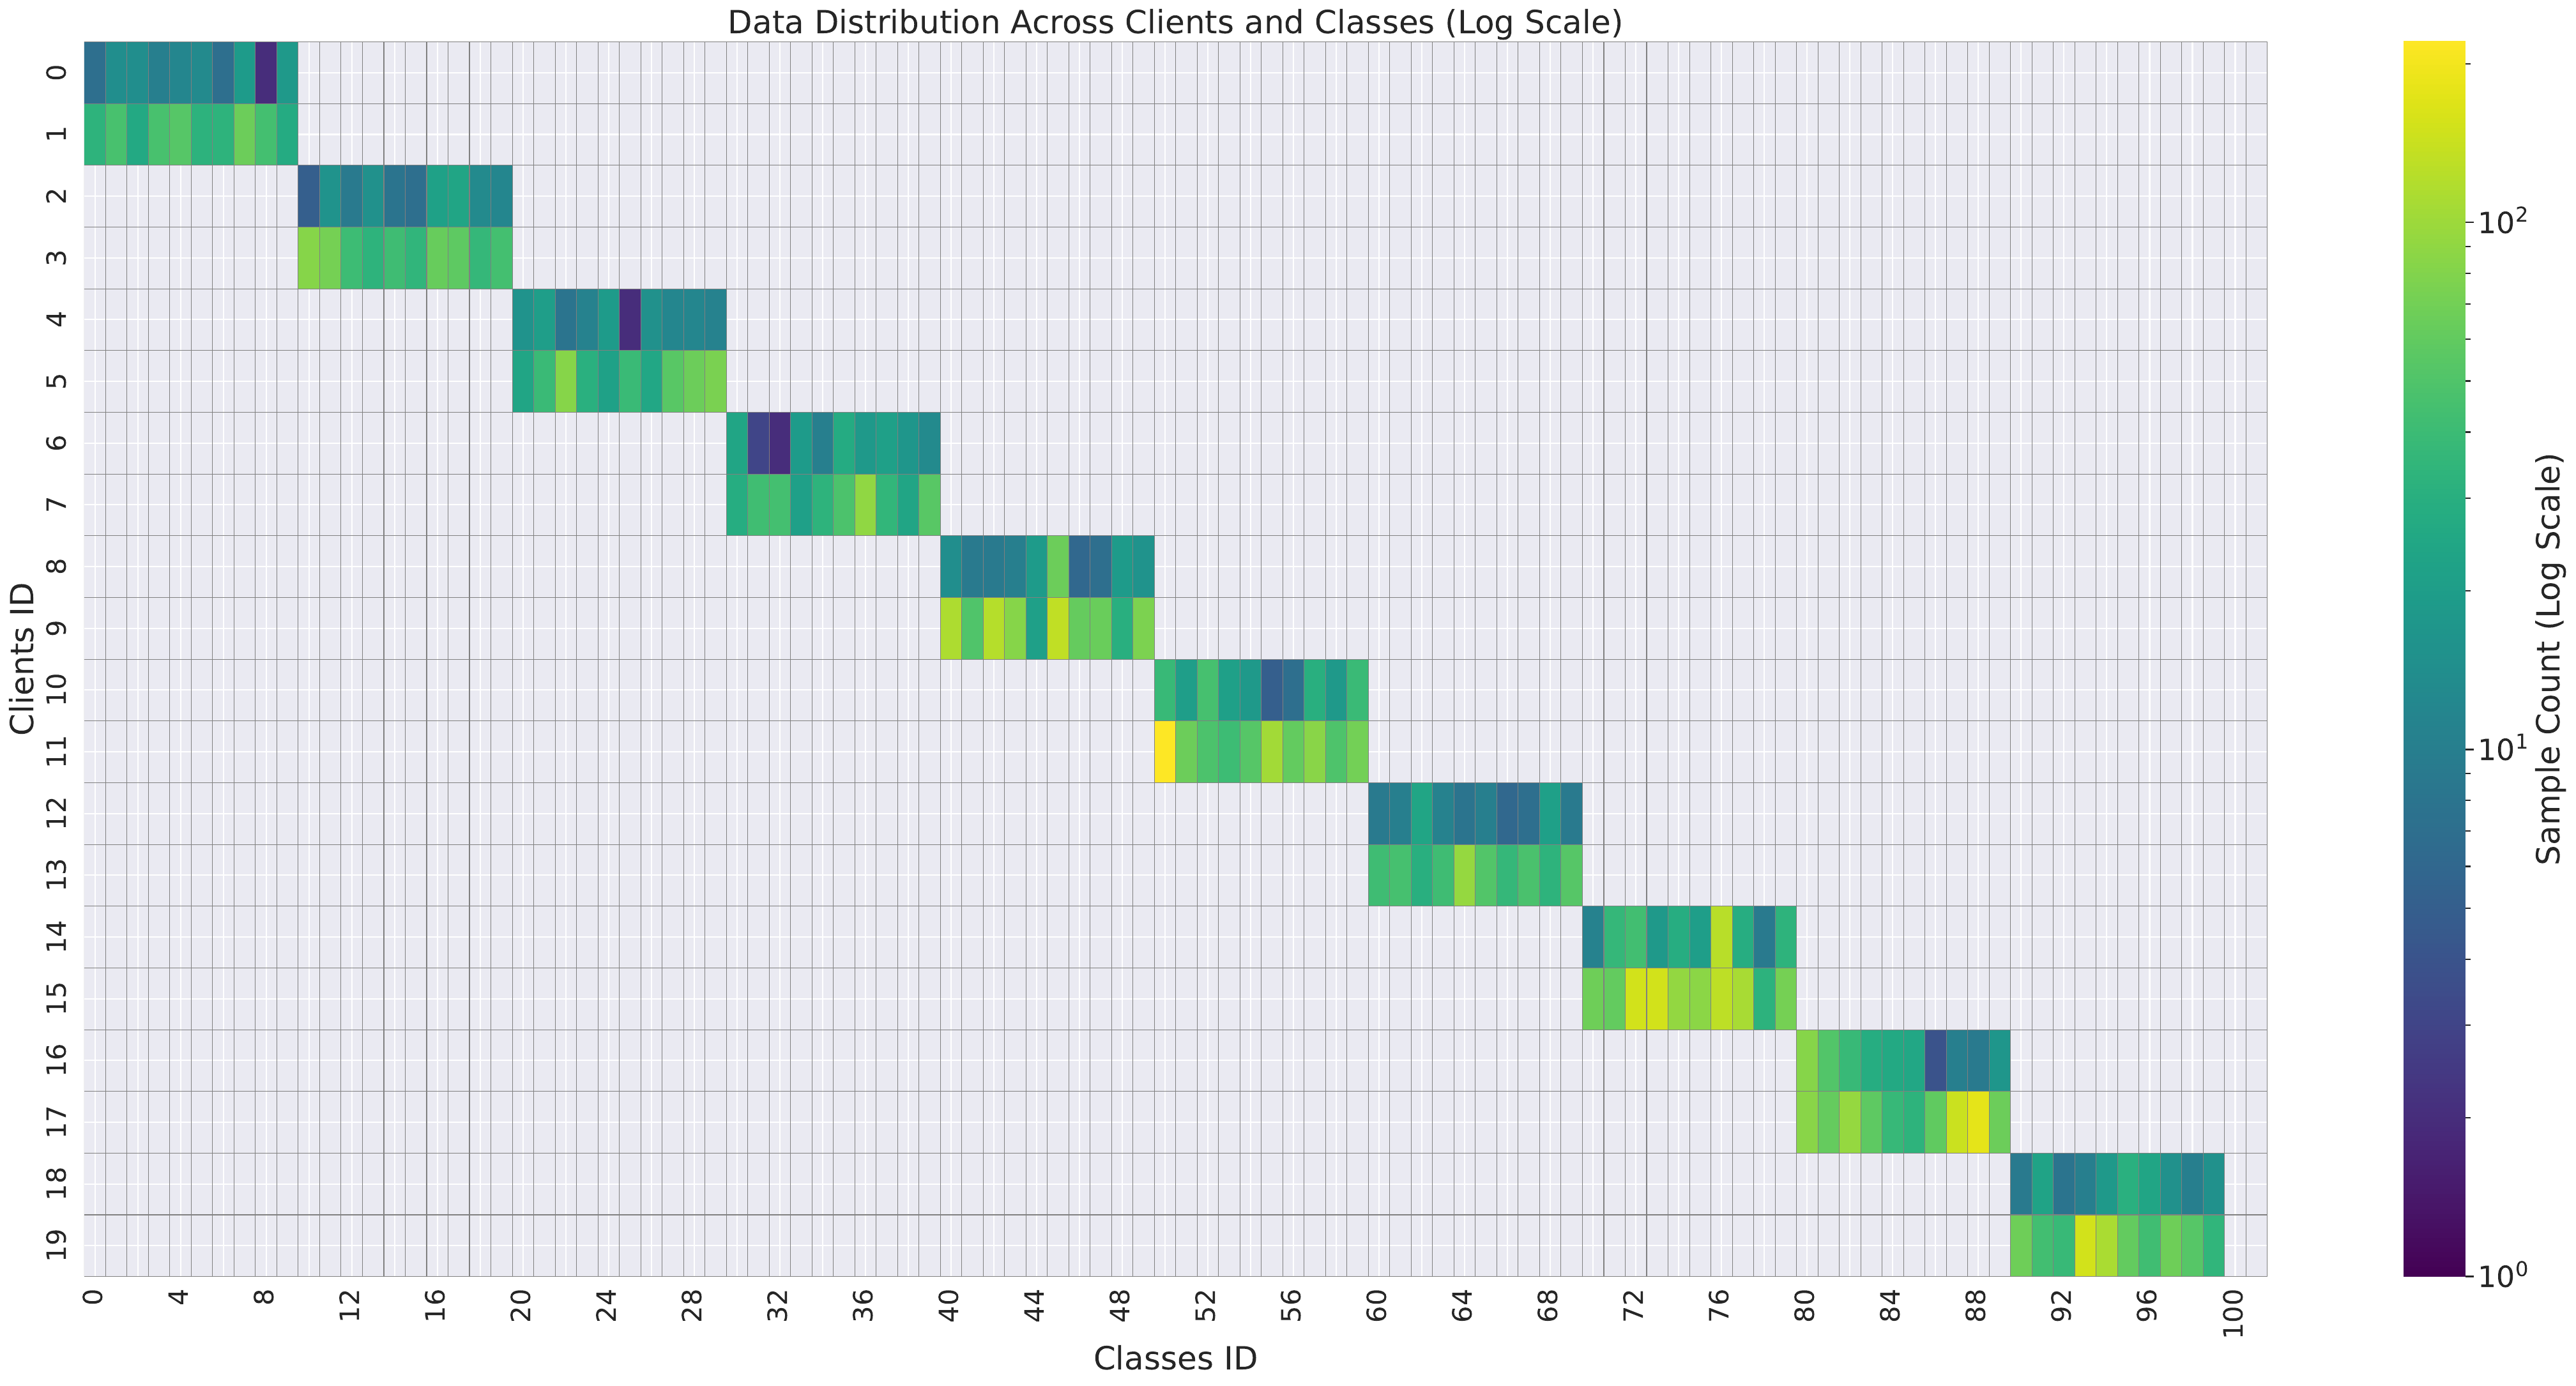}
    \caption{The data distribution for each client on the Flowers102 dataset is visualized under the pathological setting, where each client is assigned 10 classes. Brighter colors indicate larger sample sizes.}
    \label{fig:Flowers102_visualization}
\end{figure}

\begin{figure}[ht]
    \centering
    \includegraphics[width=\linewidth, height=10cm]{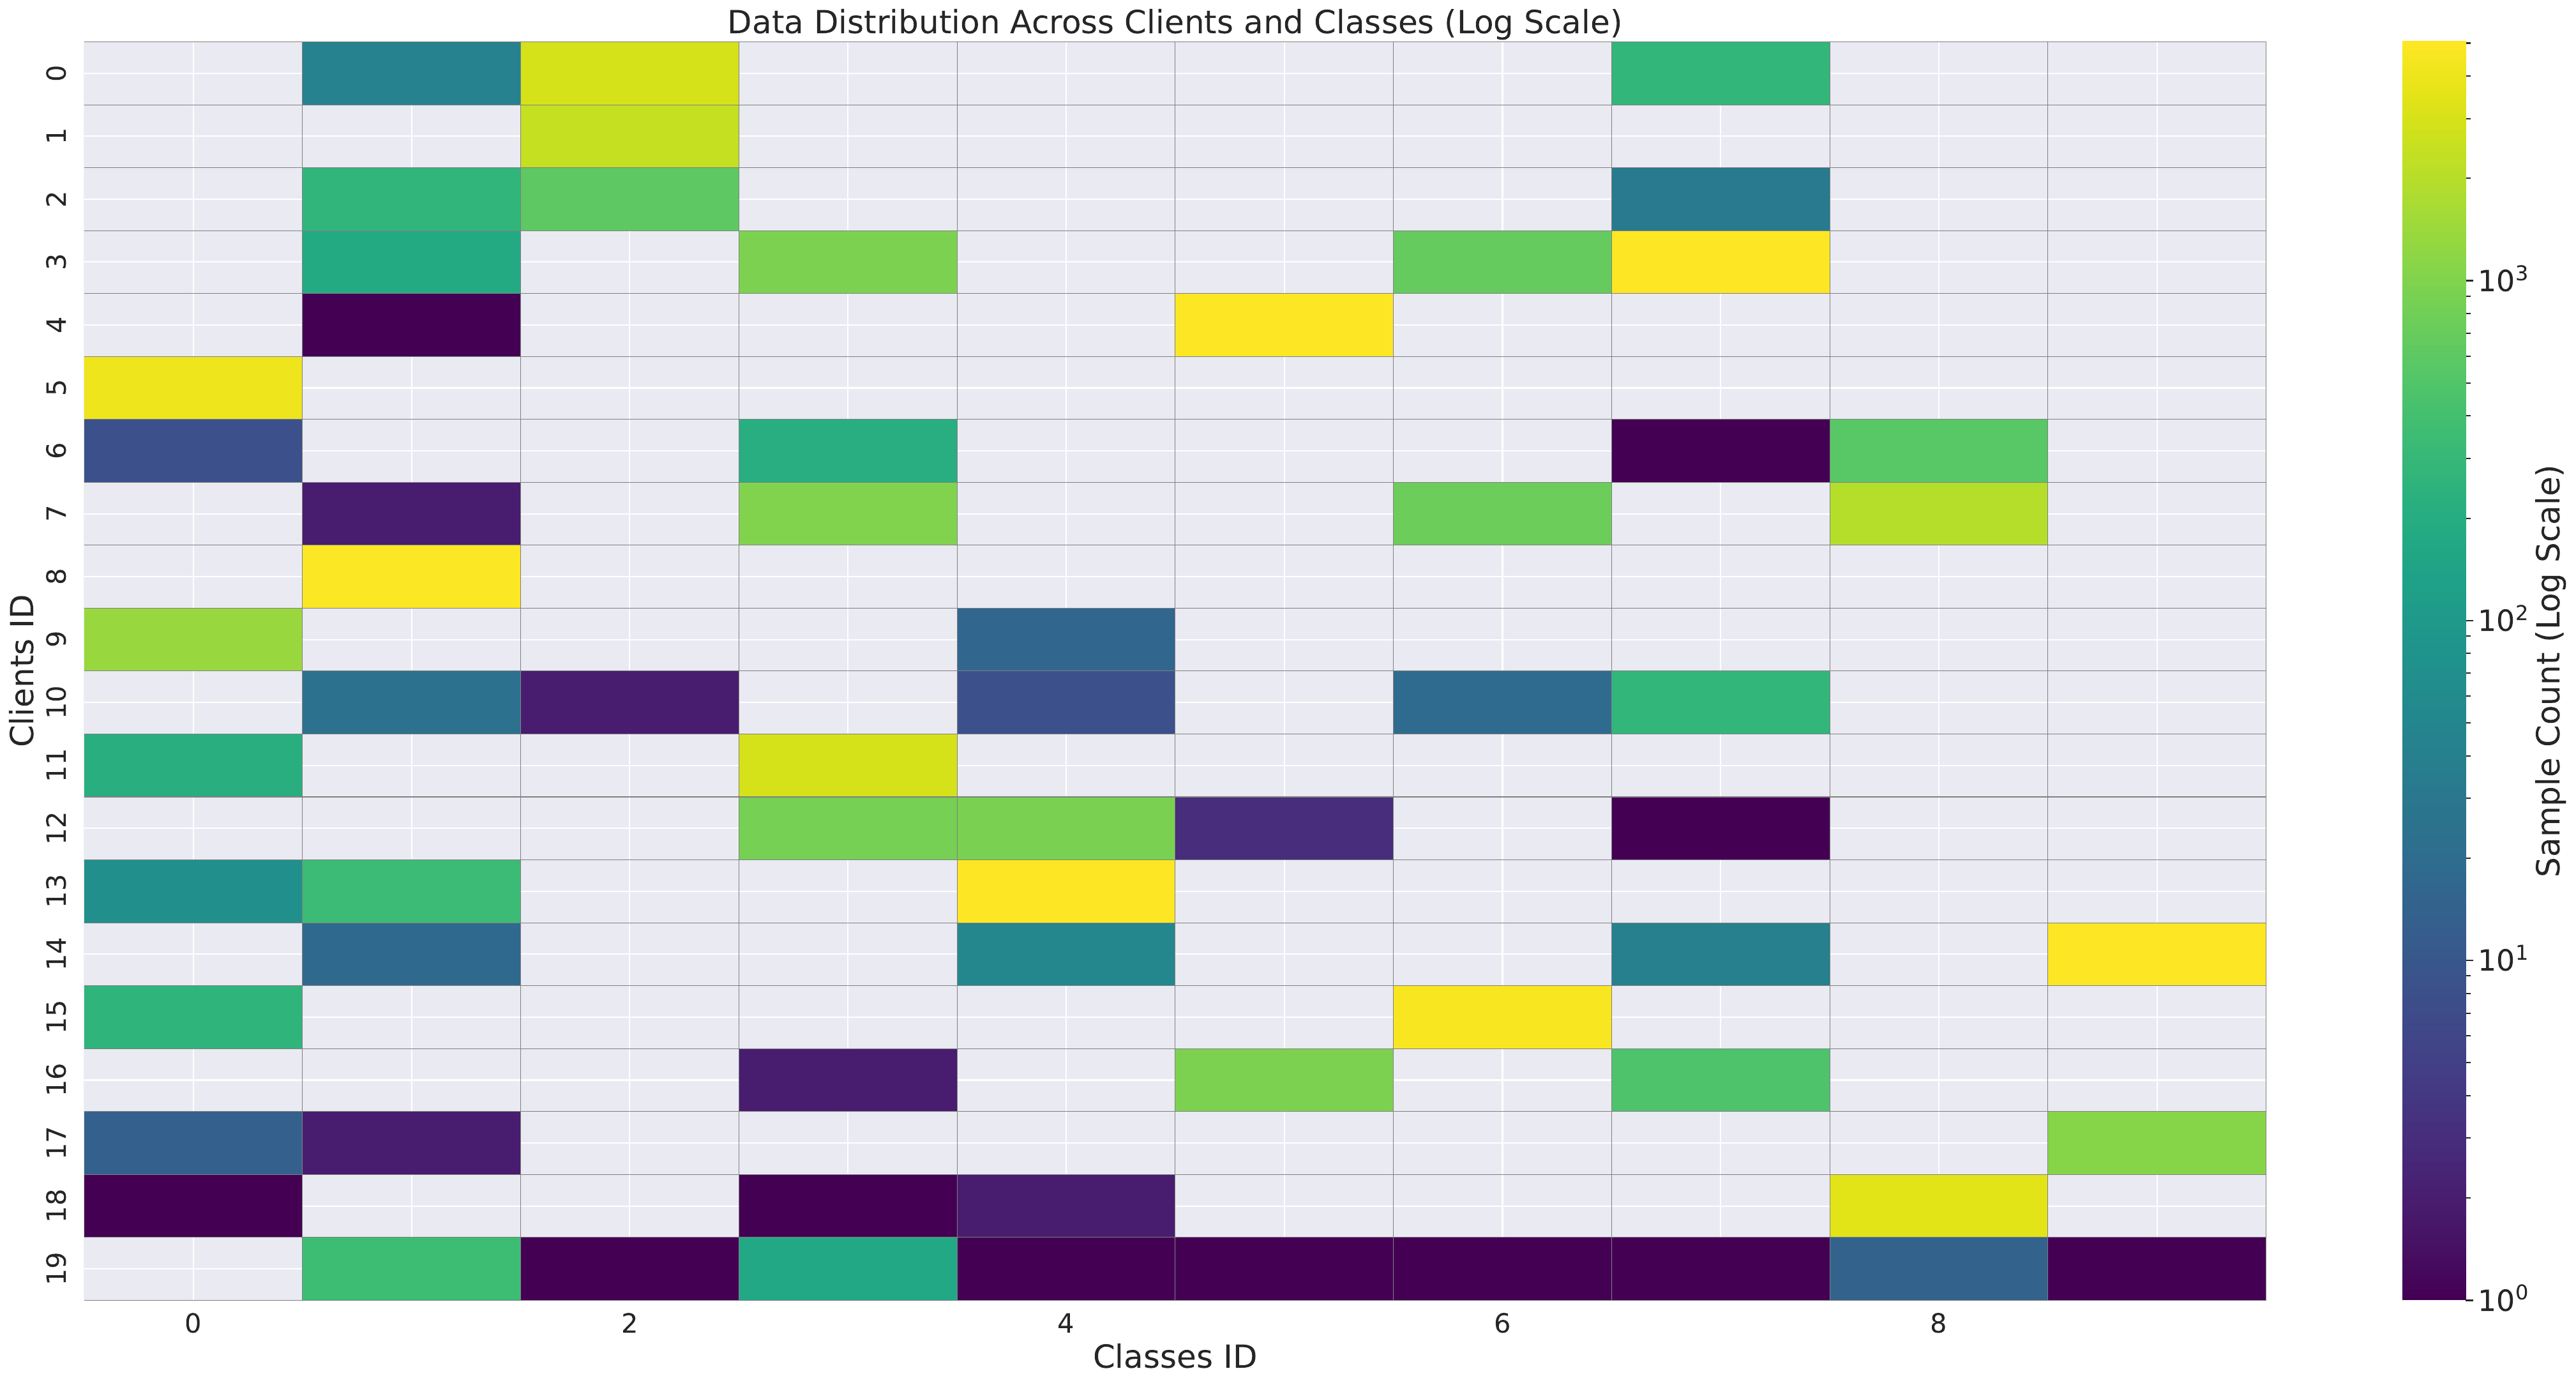}
    \caption{The data distribution for each client on the Cifar10 dataset is visualized under the practical setting (with $\alpha = 0.05$). Brighter colors indicate larger sample sizes.}
    \label{fig:Cifar10_dir0.05_visualization}
\end{figure}

\begin{figure}[ht]
    \centering
    \includegraphics[width=\linewidth, height=10cm]{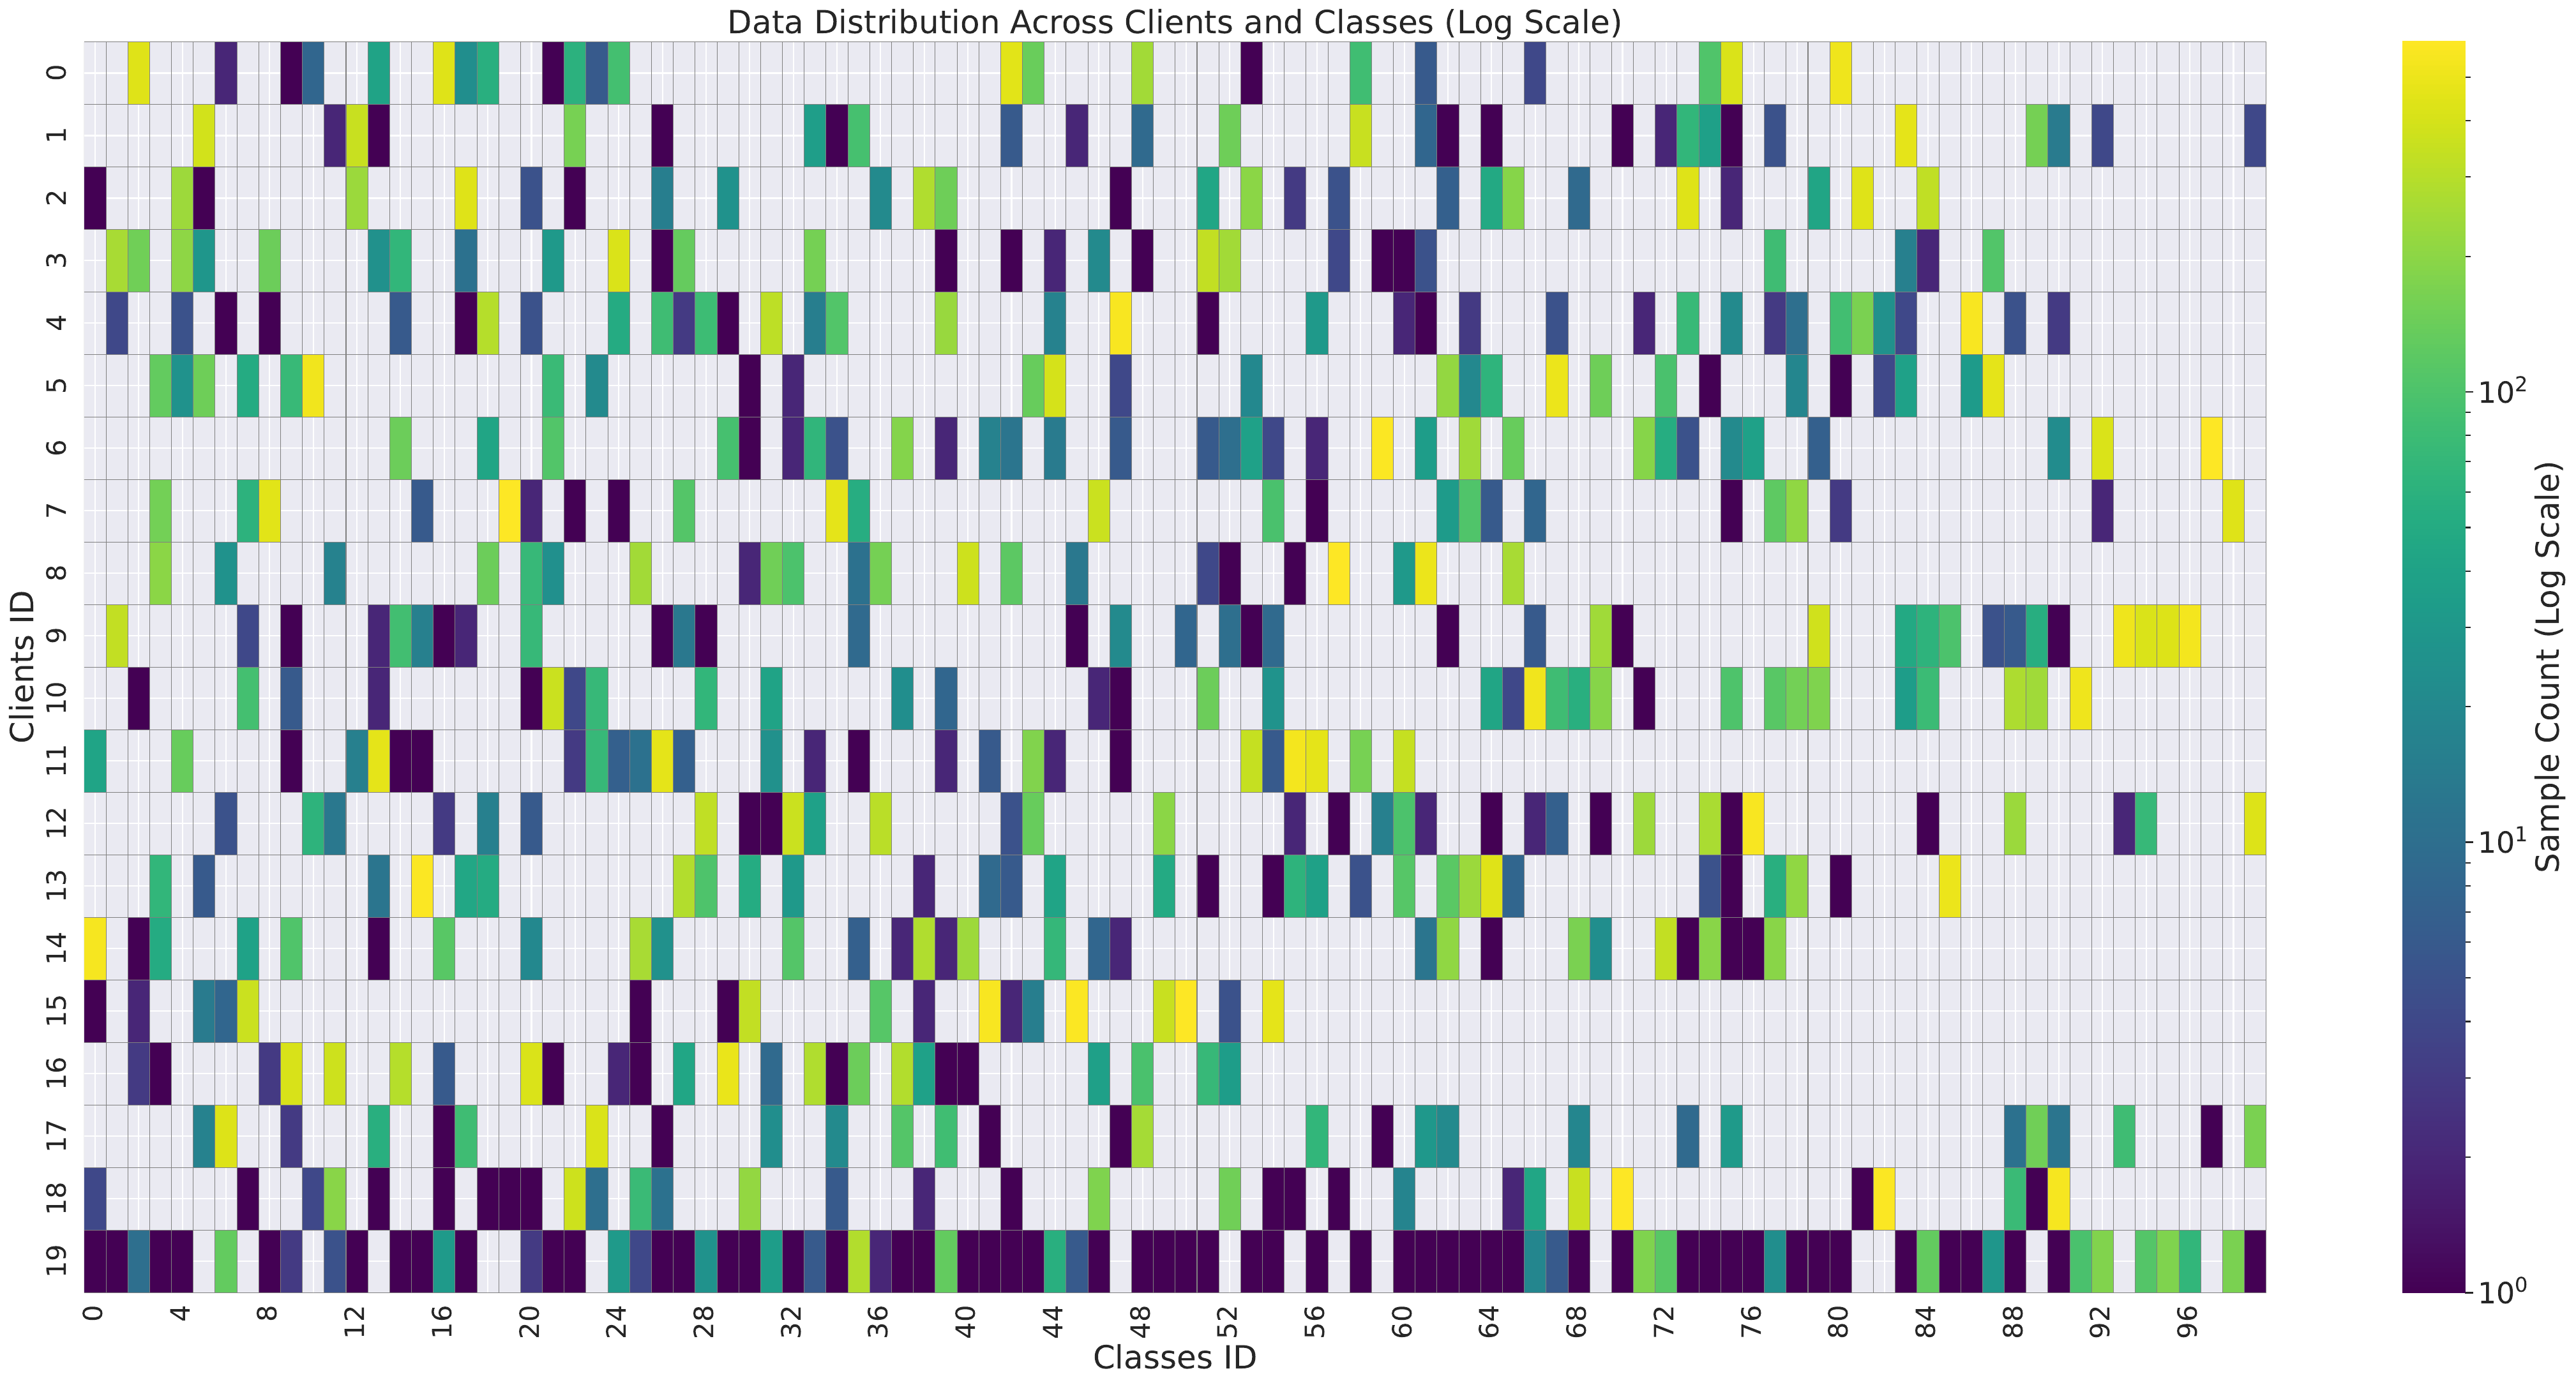}
    \caption{The data distribution for each client on the Cifar100 dataset is visualized the practical setting (with $\alpha = 0.05$). Brighter colors indicate larger sample sizes.}
    \label{fig:Cifar100_dir0.05_visualization}
\end{figure}

\begin{figure}[ht]
    \centering
    \includegraphics[width=\linewidth, height=10cm]{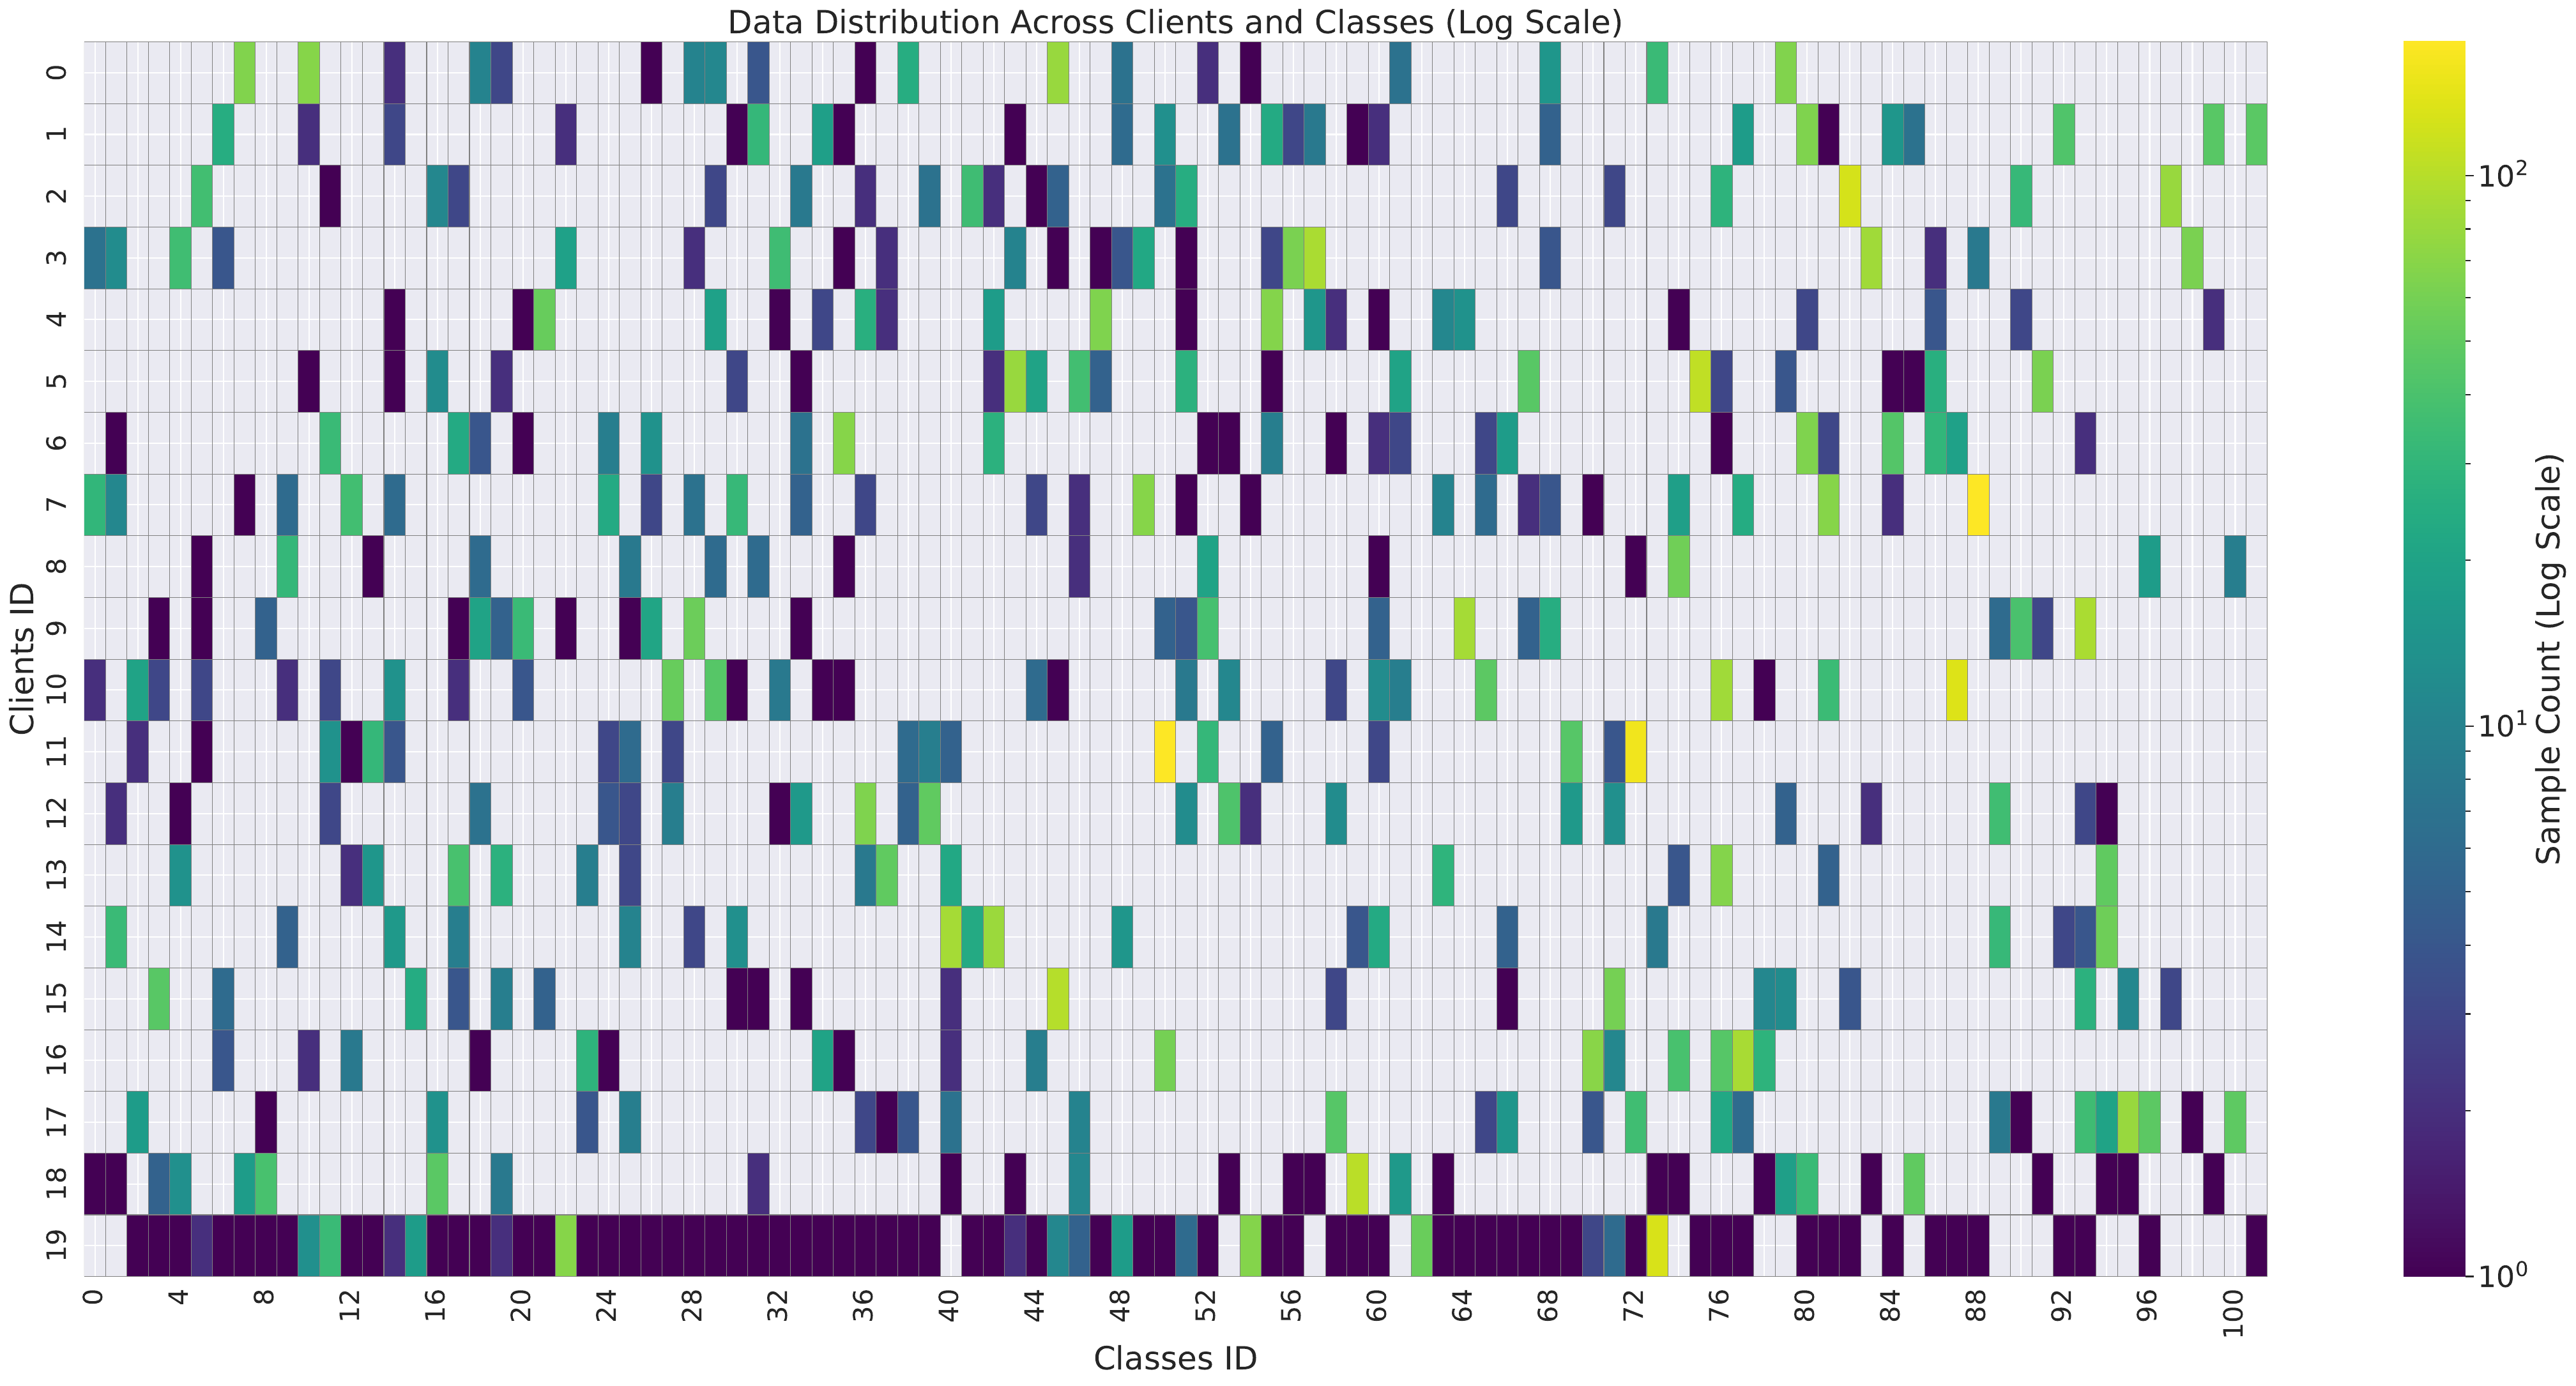}
    \caption{The data distribution for each client on the Flowers102 dataset is visualized the practical setting (with $\alpha = 0.05$). Brighter colors indicate larger sample sizes.}
    \label{fig:Flowers102_dir0.05_visualization}
\end{figure}

\begin{figure}[ht]
    \centering
    \includegraphics[width=\linewidth, height=10cm]{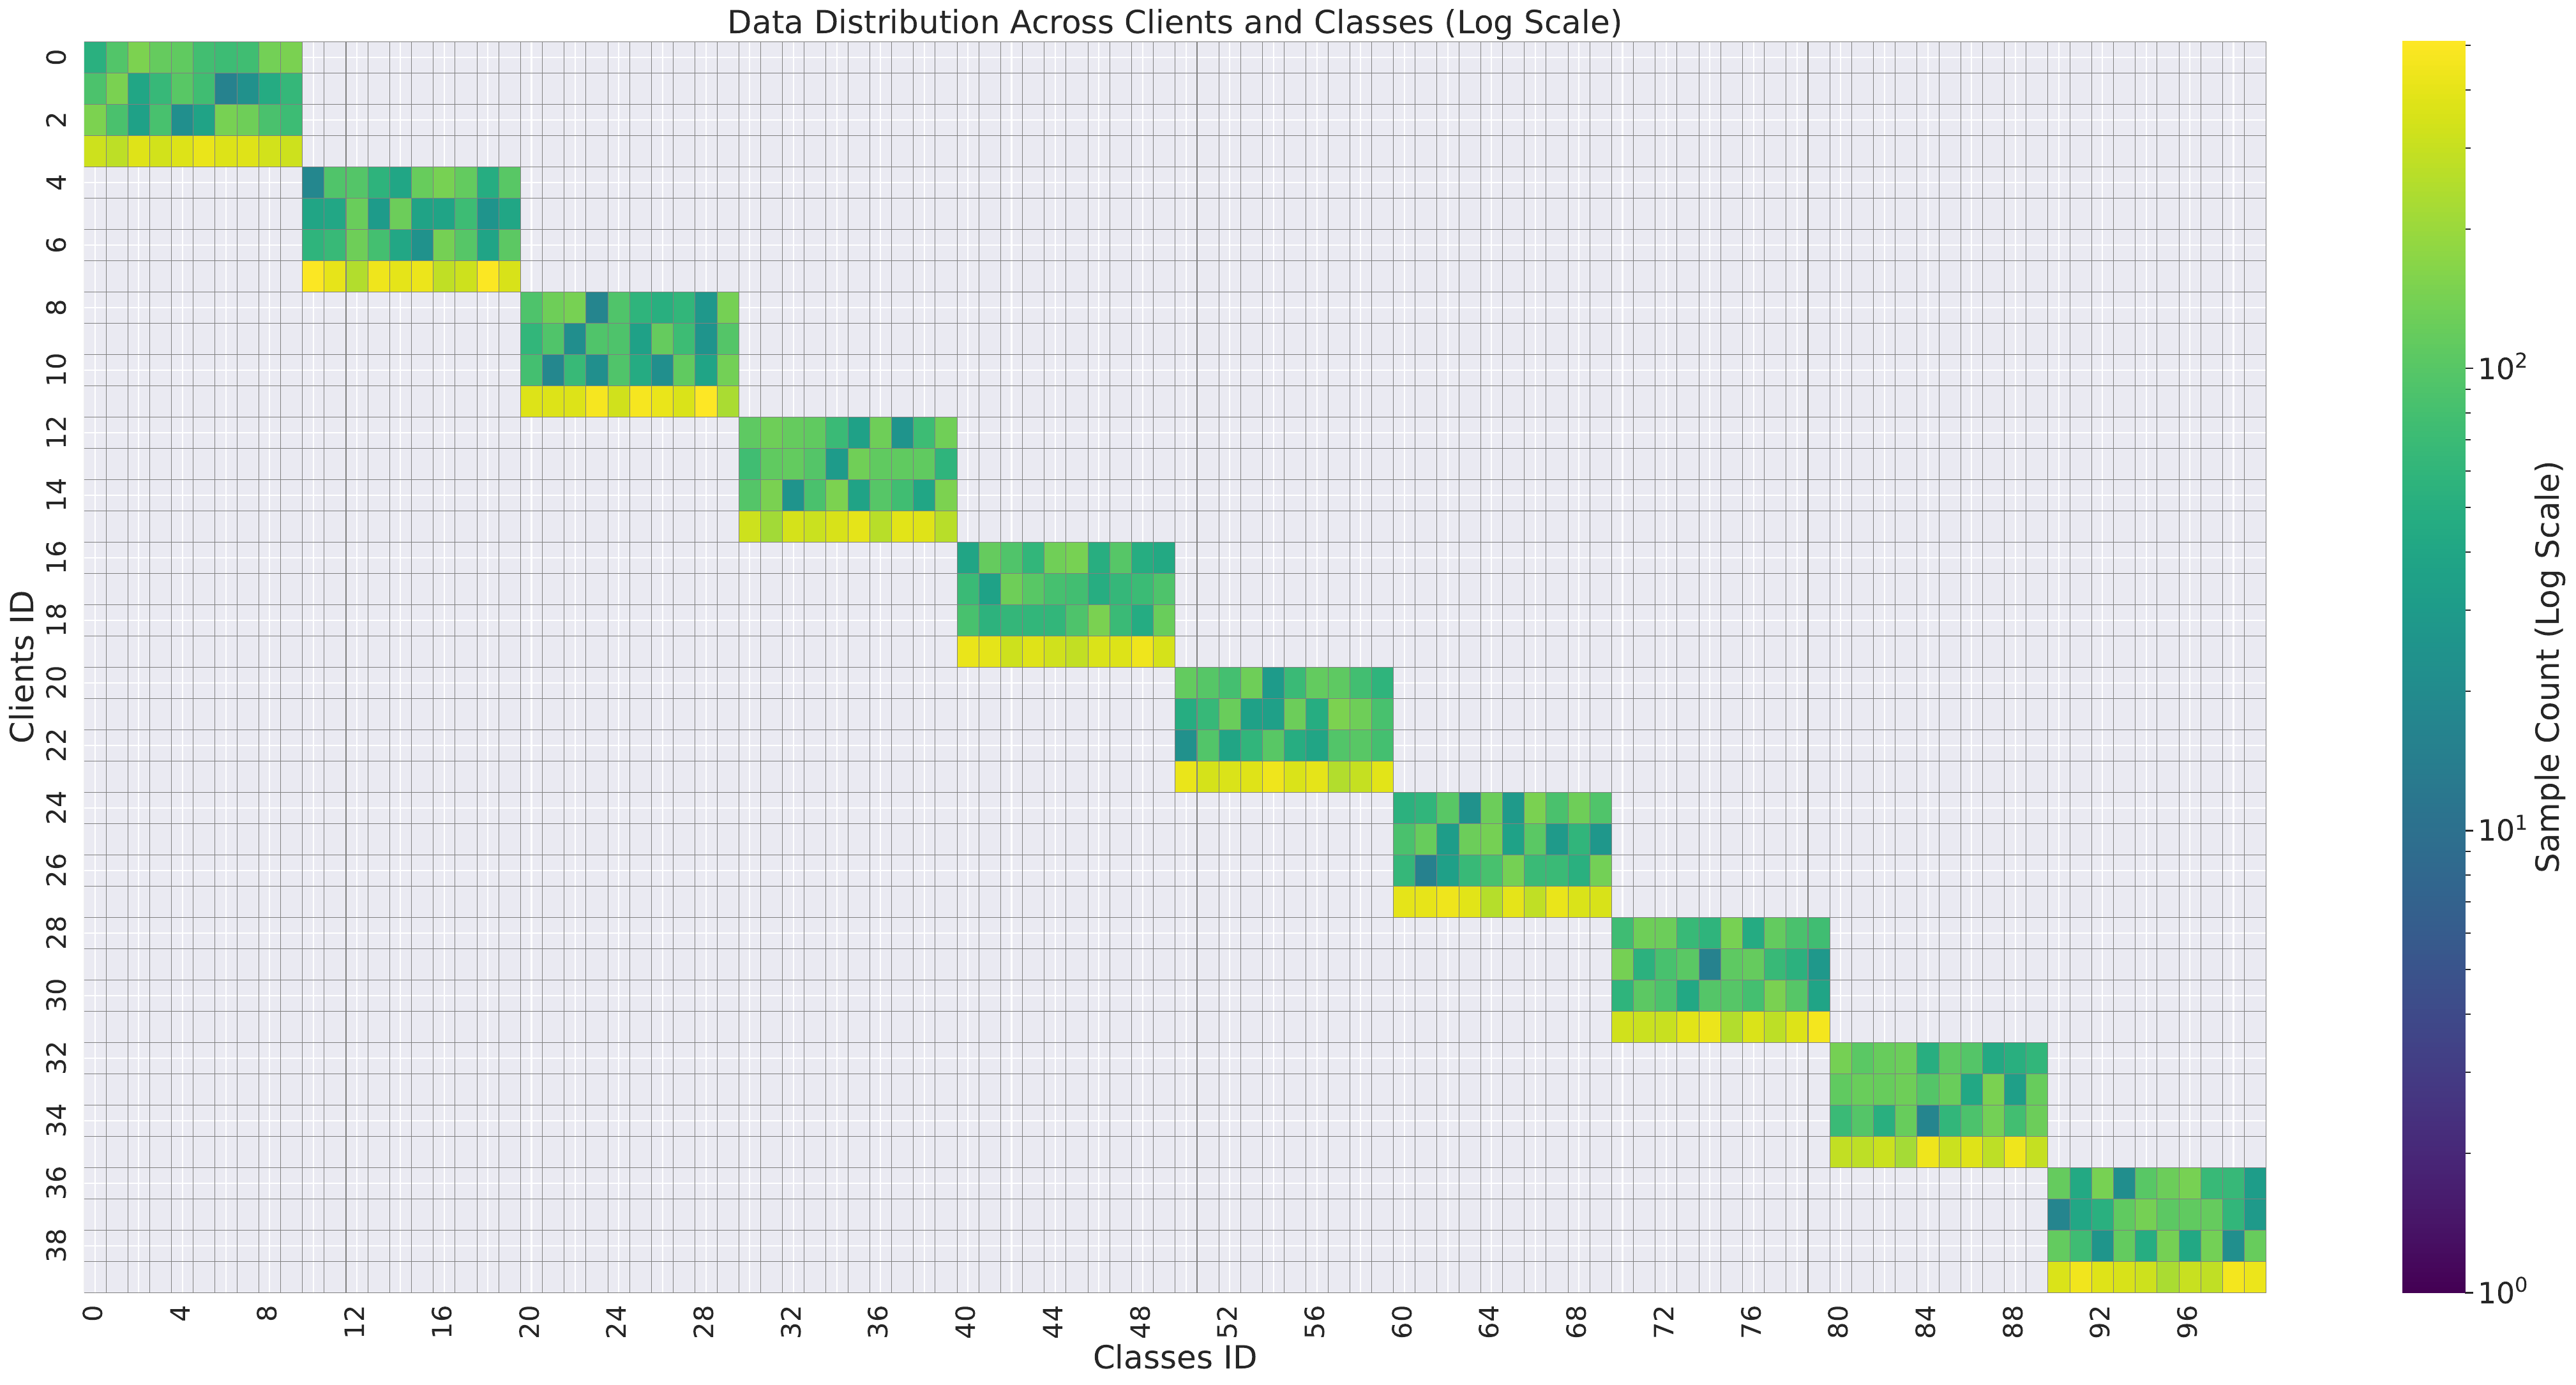}
    \caption{The data distribution for each client on the Cifar100 dataset is visualized under the various participation rate setting, where each client is assigned 10 classes. Brighter colors indicate larger sample sizes.}
    \label{fig:Cifar100_M=40_C=0.5_visualization}
\end{figure}

\begin{figure}[ht]
    \centering
    \includegraphics[width=\linewidth, height=10cm]{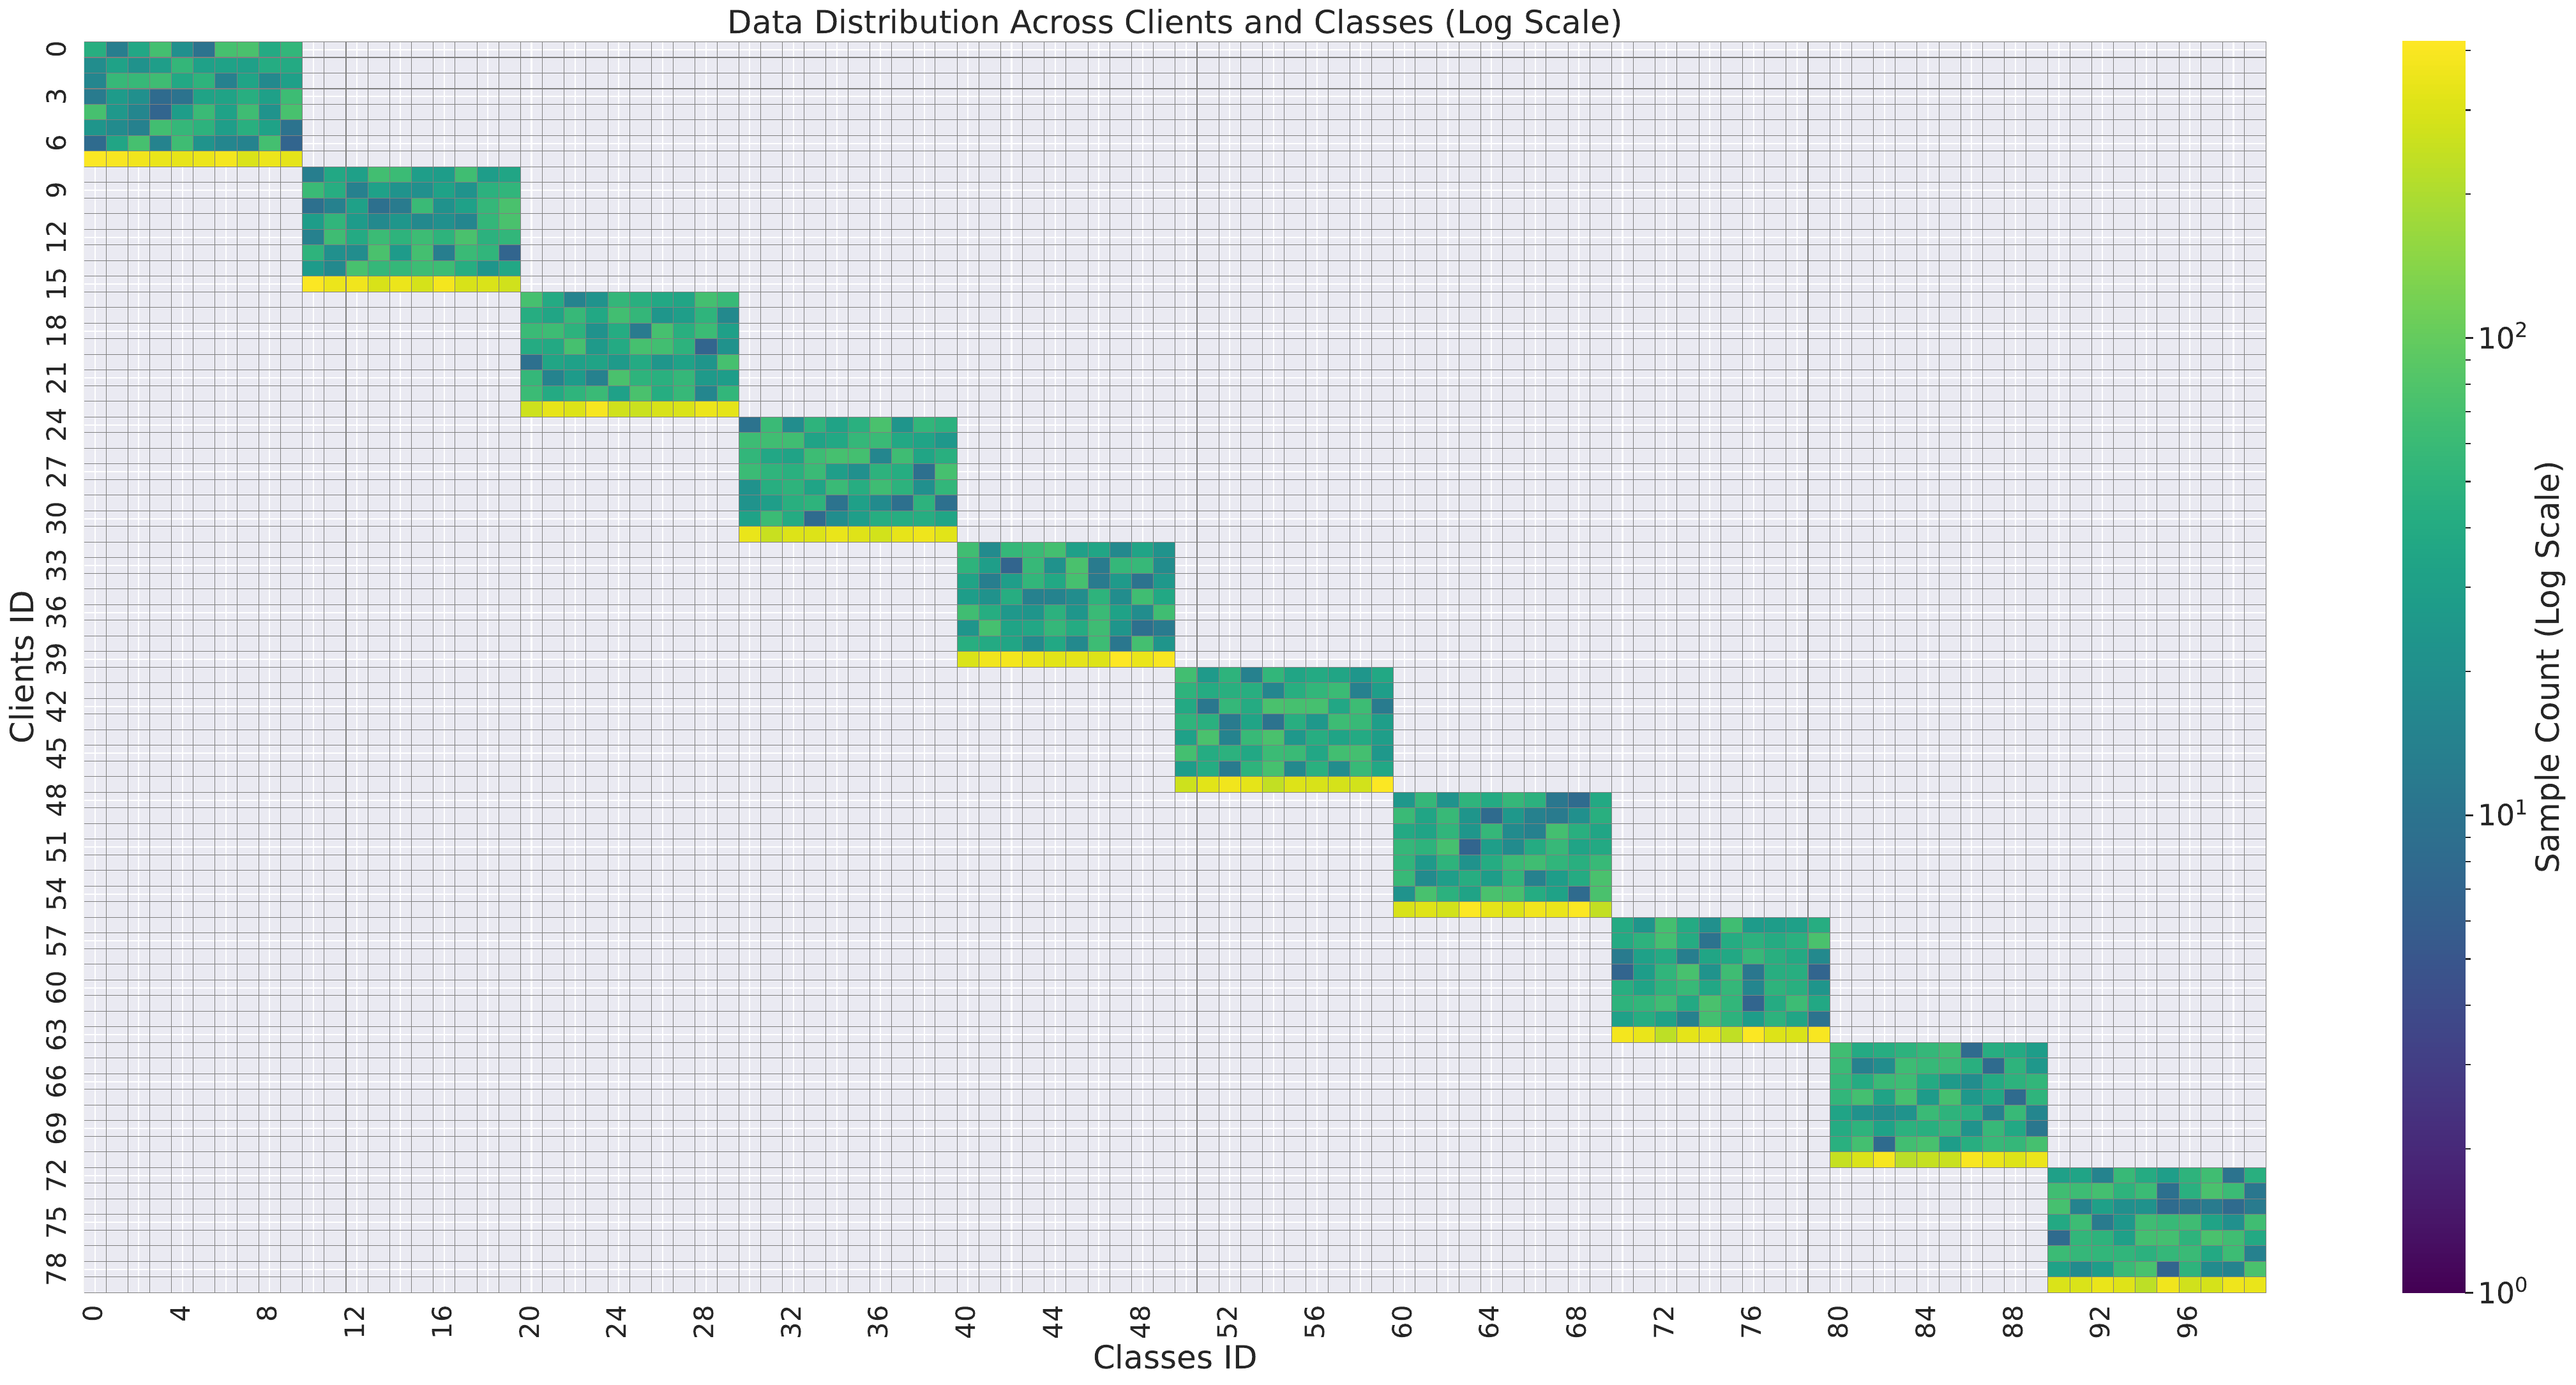}
    \caption{The data distribution for each client on the Cifar100 dataset is visualized under the various participation rate setting, where each client is assigned 10 classes. Brighter colors indicate larger sample sizes.}
    \label{fig:Cifar100_M=80_C=0.25_visualization}
\end{figure}

\begin{figure}[ht]
    \centering
    \includegraphics[width=\linewidth, height=10cm]{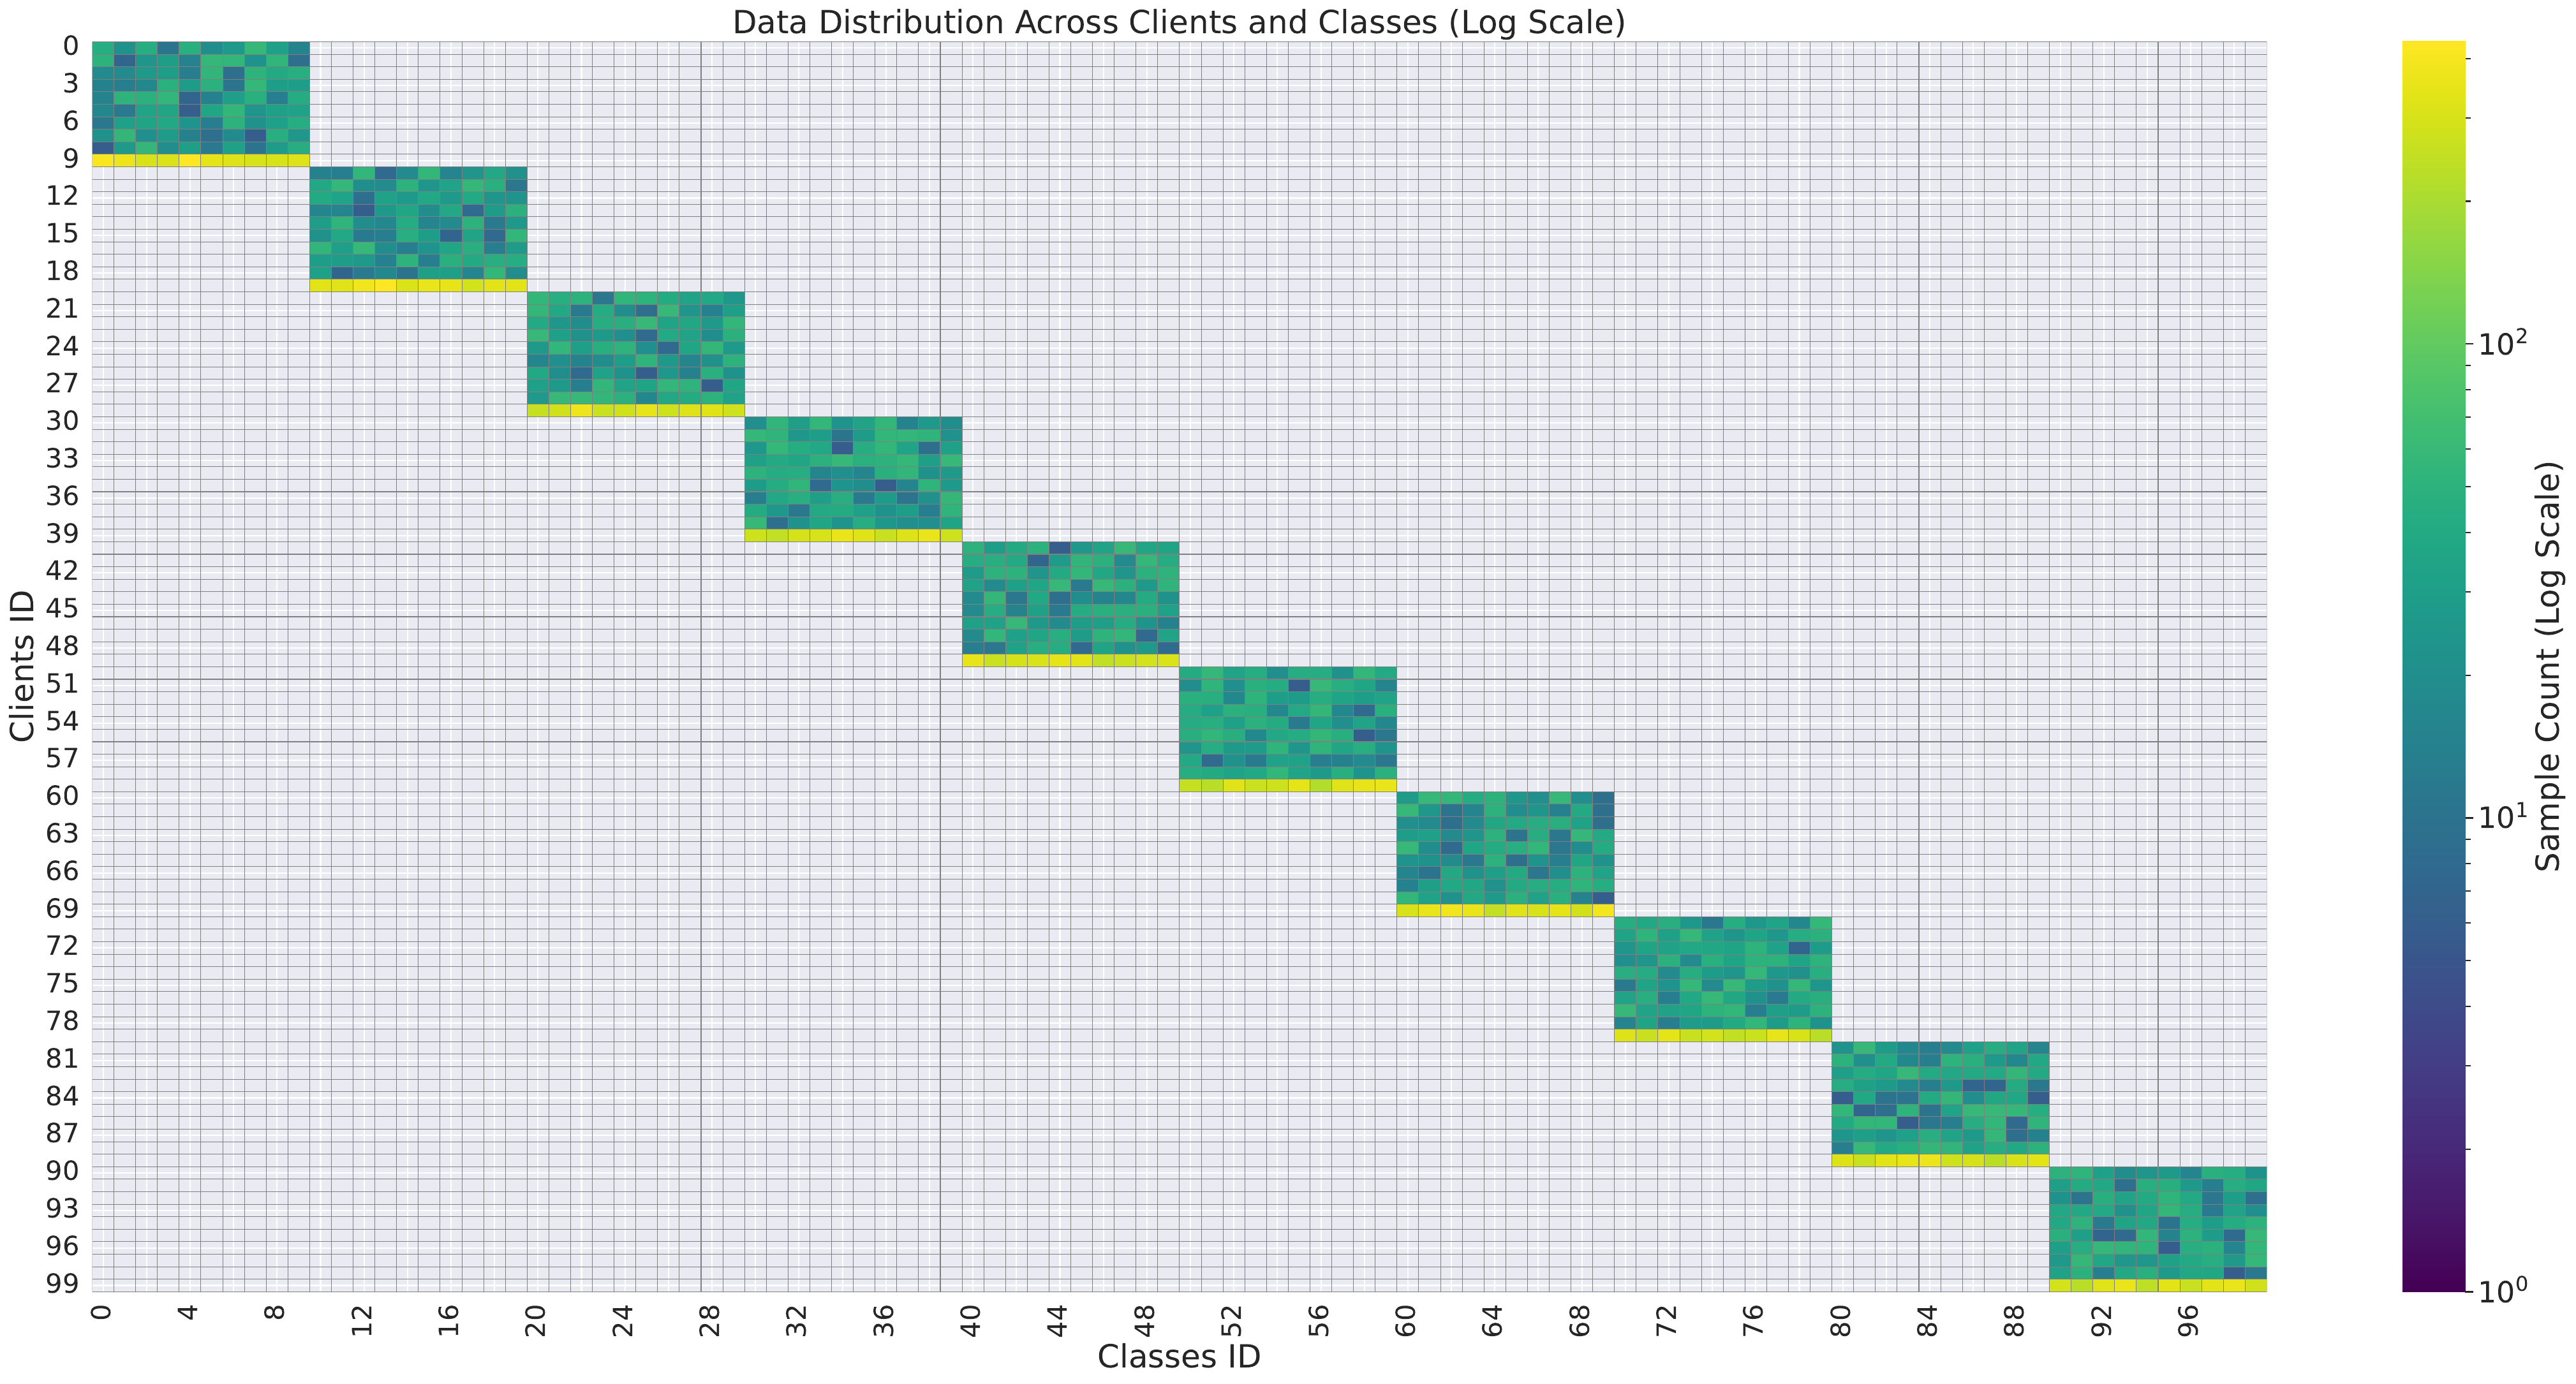}
    \caption{The data distribution for each client on the Cifar100 dataset is visualized under the various participation rate setting, where each client is assigned 10 classes. Brighter colors indicate larger sample sizes.}
    \label{fig:Cifar100_M=100_C=0.2_visualization}
\end{figure}
